# Supplementary material for: On the ratio of lapses in bimetric relativity
Source: arXiv:1903.09646 ancillary file (2019-03-22)
Supplement: Supplementary file 2 [file 01-packager.pdf]

# Bimetric equations in standard 3+1 form reduced to spherical symmetry (packager)

Mikica Kocic, created 2017-04-04, last modified 2018-06-19

**Part I** contains the common definitions. Here we create the package “**bimetric-ss-nr.m**” that contains the 3+1 split of the bimetric field equations in spherically symmetry.

**Part II** contains the verification of the expressions from the geometric mean paper. The expressions are compared to those obtained using the direct (manual) projections of the  $V_g$  and  $V_f$ . The bimetric conservation law is obtained by projecting  $\nabla V_g$  and solving for  $\partial_t p$ .

## Requirements:

Evolution of this notebook requires packages **xAct** `xCoba` and **xAct** `TexAct`.

## Changelog:

2017-04-04 Initial release with  $g^\pm$  metrics.

2017-11-21 Modified  $g^-$  and  $g^+$  metrics to  $g$  and  $\tilde{g}$ .

2017-12-05 Solved square root in 2D (1+1) bimetric case.

2017-12-06 Verification of the 3+1 decomposition relative to  $h$ .

2018-02-04 Variables harmonized with the paper.

2018-02-04 Split into two files (old variables and new variables).

2018-02-05 EoM in terms of the operator components  $K_{1,2}$  and  $\tilde{K}_{1,2}$ .

2018-02-07 Updated texNice, texPrint, and texOut.

2018-02-10 Verification of the geom-mean expressions from the paper.

2018-05-14 Calculation of  $\partial_t p$ , and verification of the bimetric conservation law.

2018-05-16 Added  $V_{\text{sign}}$  to the  $\mathcal{P}$ -functions (used in instantiateShiftedESP) and verified  $V_{\text{sign}} = \pm 1$ .

2018-05-18 Convention where uninstantiated variables are prefixed with “eq\$” (likegBeta = eq\$gBeta).

2018-06-19 An option for the regularized  $B$  and  $\tilde{B}$  on export bimetric-ss-nr.m (multiplied with  $r$ ).

# Part I -- Create the package “bimetric-ss-nr.m”

## Definitions

### Load xAct

```
SetDirectory[NotebookDirectory[]];

Block[{Print}, Print[e_] := Null;
  << xAct`xCoba`;
  << xAct`TeXAct`;
]
```

### Configuration

Deactivate info messages in xTensor:

```
$Info = False;
```

Deactivate info messages in xCoba:

```
$CVVerbose = False;
```

Deactivate definition messages:

```
$DefInfoQ = False;
```

Hide ugly dummies:

```
$PrePrint = xAct`xTensor`ScreenDollarIndices;
```

The  $V$ -sign convention:

```
$Vsign = -1;
```

The  $K$ -sign convention is fixed to  $-1$ .

## Operators

### $\overset{k}{A}$ -- matrix power

```
 $\overset{k}{A}$ ?MatrixQ := MatrixPower[A, k]
```

### $A \cdot B$ -- matrix multiplication

```
matrixToScalar[expr_] := If[Dimensions@expr === {1, 1}, expr[[1, 1]], expr]

CenterDot[A_, 0] := ConstantArray[0, Dimensions@A] // matrixToScalar
CenterDot[0, A_] := ConstantArray[0, Dimensions@A] // matrixToScalar
CenterDot[A_, B_] := Dot[A, B] // matrixToScalar

Attributes[CenterDot] = {Flat, OneIdentity};
```

Fix the case when we have a matrix multiplication by a zero scalar,

```
Unprotect@Dot;
Dot[A_, 0] := ConstantArray[0, Dimensions@A]
Dot[0, A_] := ConstantArray[0, Dimensions@A]
Protect@Dot;
```

### □ -- flatten a partitioned matrix

```
□x_ := ArrayFlatten[x]
```

### ▼ -- get the spatial part of a matrix or a vector

```
▼[expr_?MatrixQ] := If[Dimensions[expr][[2]] == 1, expr[[2 ;; All]],
  If[Dimensions[expr][[1]] == 1, expr[[1, 2 ;; All], expr[[2 ;; All, 2 ;; All]]]]
▼[expr_?ListQ] := expr[[2 ;; All]]
```

### ⊕ -- direct sum of matrices

```
ClearAll@CirclePlus
CirclePlus[a_, b_] := ArrayFlatten@{{a, 0}, {0, CirclePlus[b]}}
CirclePlus[a_] := a
```

### diag -- diagonal matrix of elements

```
diag[e_, n_] := DiagonalMatrix@Table[e, n]
```

### $\mathcal{E}_n$ -- elementary symmetric polynomial (ESP)

```
 $\mathcal{E}_n[X_] := If[n < 0 \vee n > Length@X, 0,
  SymmetricPolynomial[n, Eigenvalues[X]]
]$ 
```

### $\mathcal{Y}_n$ -- derivative of ESP

```
 $\mathcal{Y}_n[X_] := If[n < 0 \vee n \geq Length@X, 0,
  If[n == 0, IdentityMatrix[Length@X],
    \sum_{k=0}^n (-1)^{n+k} \mathcal{E}_k[X] \frac{\partial}{\partial X^{n-k}}
  ]]$ 
```

### $\langle X \rangle_k^n$ -- shifted elementary symmetric polynomial

```
Tex[P[n_, k_, F_]] := "\\left\\langle" <> Tex@F <> "\\right\\rangle" <> Tex@n <> "_" <> Tex@k
```

Utility to instantiate the deformed symmetric polynomials,

```
instantiateShiftedESP[e_] := e //. {P[d_, k_, x_] => P[d, k, x]}
P[n_, k_, S_?MatrixQ] := Sum[
  $Vsign  $\beta$ [i + k] SymmetricPolynomial[i, Eigenvalues[S]],
  {i, 0, n}
]
```

```

P[n_, k_, ev_List] := Sum[
  $Vsign β[i + k] SymmetricPolynomial[i, ev],
  {i, 0, n}
]

P[n_, k_, ev_] := Sum[
  $Vsign β[i + k] SymmetricPolynomial[i, Table[ev, n]],
  {i, 0, n}
]

PP[n_, k_, λ_, k2_, λ2_] := ∑i=0k2 P[n, k + i, λ] SymmetricPolynomial[i, Table[λ2, k2]]

```

## Utility functions

`printNice` -- print tensorial expression in a nice form

```

printNice[e_, extra_ : {ff_[t, r] => ff, ff_[t] => ff, ff_[r] => ff}] := e //. {
  gEA → Style[A, Blue], gEB → Style[B, Blue], gK1 → Style[K1, Blue],
  gK2 → Style[K2, Blue], gAlpha → Style[α, Blue], gBeta → Style[β, Blue],
  fEA → Style[Ã, Red], fEB → Style[Ḃ, Red], fK1 → Style[Ḳ1, Red],
  fK2 → Style[Ḳ2, Red], fAlpha → Style[ἄ, Red], fBeta → Style[ḃ, Red],
  sER → Style[R, Magenta], hBeta → Style[q, Darker@Green], rhoPF → Style[ρPF, Purple],
  sLp → Style[p, Darker@Green],
  sLv → Style[v, Darker@Green], sLt → Style[λ, Darker@Green],
  k$g → Style[kg, Blue], k$f → Style[kf, Red], β[n_] => βn,
  (***)
  P[d_, k_, x_List] => HoldForm[⟨Sequence@@x⟩kd],
  P[d_, k_, x___] => HoldForm[⟨x⟩kd],
  t[] → t, r[] → r, θ[] → θ, φ[] → φ
} //. {
  Derivative[n1_, n2_][f_][x1_, x2_] => sp$der[f[x1, x2] /. extra, {{n1, x1}, {n2, x2}}],
  Derivative[n1_, n2_, n3_][f_][x1_, x2_, x3_] =>
    sp$der[f[x1, x2, x3] /. extra, {{n1, x1}, {n2, x2}, {n3, x3}}],
  Derivative[n1_, n2_, n3_, n4_][f_][x1_, x2_, x3_, x4_] =>
    sp$der[f[x1, x2, x3, x4] /. extra, {{n1, x1}, {n2, x2}, {n3, x3}, {n4, x4}}]
} //.
extra

sp$der[f_, nx_] :=
  DisplayForm@TagBox[RowBox[{SubscriptBox["∂", StyleBox[RowBox@Flatten[
    If[#[[1]] == 0, Nothing, Table[ToBoxes@printNice@#[[2]], #[[1]]]] & /@ nx
  ], Red]], "", ToBoxes[f]]], HoldForm]

printHeader[e_] := CellPrint@Cell[DisplayForm@e, "Text", FontFamily → "Cambria",
  CellFrame → {{1, 0}, {0, 0.1}}, CellMargins -> {{34, 0}, {Inherited, Inherited}}]

```

## filterNonZeroNonEqual -- filter redundant equations

```

filterNonZeroNonEqual[exprList_] := Module[
  {es = {0}, e = Flatten@exprList},
  Do[
    If[Not@MemberQ[Simplify[Join[Thread[es - e[[i]], Thread[es + e[[i]]]], 0],
      AppendTo[es, e[[i]]]
    ],
    {i, Length@e}
  ];
  es[[2 ;;]]

printNonzeroEqs[method_][e_] := Block[
  {allZero = True},
  Do[
    If[e[[i$N]] != 0, allZero = False;
    Echo[method[e[[i$N]]], ToString[i$N] <> ": "];
  ],
  {i$N, 1, Length@e}
];
If[allZero, Echo["All equations are zero"]]
]

```

## densitize\$lapse -- redefine lapses

```

densitize$lapse[expr_] := Block[
  {gAlpha, fAlpha},
  gAlpha[t_, r_] := gAlpha2[t, r] gEA[t, r];
  fAlpha[t_, r_] := fAlpha2[t, r] fEA[t, r];
  expr
] /. {gAlpha2 → gAlpha, fAlpha2 → fAlpha} // Simplify

```

## convert\$K -- redefine K variables

```

convert$K[expr_] := Block[
  {gKr, gKθ, fKr, fKθ},
  gKr[t_, r_] := gEA[t, r]^2 gK1[t, r];
  gKθ[t_, r_] := gEB[t, r]^2 gK2[t, r];
  fKr[t_, r_] := fEA[t, r]^2 fK1[t, r];
  fKθ[t_, r_] := fEB[t, r]^2 fK2[t, r];
  expr // Simplify
]

```

## simplifyShiftedESP -- recognize shifted ESP

```

simplifyShiftedESP[expr_] := Block[
  {$Assumptions, e2, countBeta, countP, newP},
  e2 = expr /. {fEB[t_, r_] => gEB[t, r] sER[t, r]};
  countBeta = 0; e2 /. {β[n_] => (countBeta++)};
  countP = 0; e2 /. {P[n_, k_, x_] => (countP++)};
  If[countBeta > 0 && countP > 0, Print["#β[] > 0 and #P[] > 0"]; Abort[]];
  If[countBeta > 0,
    $Assumptions =
      P[1, 0, sER] == β[0] + β[1] sER &&
      P[1, 1, sER] == β[1] + β[2] sER &&
      P[1, 2, sER] == β[2] + β[3] sER &&
      P[1, 3, sER] == β[3] + β[4] sER;
    e2 = e2 // FullSimplify;
  ];
  newP = 0; e2 /. {P[n_, k_, x_] => (newP++)};
  If[newP > 0,
    $Assumptions =
      P[2, 0, sER] == P[1, 0, sER] + P[1, 1, sER] sER &&
      P[2, 1, sER] == P[1, 1, sER] + P[1, 2, sER] sER &&
      P[2, 2, sER] == P[1, 2, sER] + P[1, 3, sER] sER;
    e2 = e2 // FullSimplify;
  ];
  (* change the sign of V, if there were betas *)
  If[countBeta > 0,
    e2 = e2 /. {P[n_, k_, x_] => $Vsign P[n, k, x]};
  ];
  e2 // Simplify
]

```

## convert\$*p2λ* -- convert boost *p* to Lorentz factor *λ*

```

convert$p2λ[expr_] := Block[{e2},
  e2 = expr /. {sLp -> (sLt2 - 1)1/2} // Simplify;
  e2 /.  $\sqrt{-1 + \underline{sLt}^2} \rightarrow \underline{sLp}$  // FullSimplify
]

```

## Manifold, chart, and scalar fields

### $\Sigma_t$ -- Manifold with the abstract indices *i*, *j*, *k*, *ℓ*

```
DefManifold[Σt, 3, {i, j, k, ℓ}]
```

### $\gamma_{ij}$ -- Spatial metric

```

DefMetric[1, γ[-i, -j], cdg, SymbolOfCovD -> {"|", "D"}, PrintAs -> "γ"];
Tex[γ] := "\\gSp";
Tex[Riccicdg] := "\\gR";
Tex[cdg] := "\\gD";

```

## $\varphi_{ij}$ -- Spatial metric

```
Off[DefMetric::old]

DefMetric[1,  $\varphi[-i, -j]$ , cdf, SymbolOfCovD -> {"", "D"}, PrintAs -> " $\varphi$ "];
Tex[ $\varphi$ ] := "\\fSp";
Tex[Riccicdf] := "\\fR";
Tex[cdf] := "\\fD";
```

## $\Sigma_B$ -- Chart ( $r, \theta, \phi$ ) on the spatial slice

```
DefChart[ $\Sigma_B$ ,  $\Sigma_t$ , Range[1, 3], { $r[]$ ,  $\theta[]$ ,  $\phi[]$ }, ChartColor -> RGBColor[0, 0.7, 0]]
```

Convert coordinate index (numbers) to a string,

```
coordToString[ $i_$ ] := {"r", " $\theta$ ", " $\phi$ "}[[ $i$ ]]
coordToString[ $i_$ ,  $j_$ ] := coordToString[ $i$ ] <> coordToString[ $j$ ]
```

Extra time coordinate (ignored by spatial derivatives),

```
DefTensor[t[], {}, PrintAs -> "t"]
cdg[ $n_$ ][t[]] := 0
cdf[ $n_$ ][t[]] := 0
```

Expand the tensorial expression in the basis  $\Sigma_B$ ,

```
toB[expr_] :=
  expr // ToBasis[ $\Sigma_B$ ] // ToBasis[ $\Sigma_B$ ] // TraceBasisDummy // ComponentArray // ToValues //
  Simplify
```

Specify components of a vector  $v^i$

```
allCV[v_, v#, metric_, post_: (# &)] := Block[{},
  AllComponentValues[v[{ $i$ ,  $\Sigma_B$ }], v# // post];
  AllComponentValues[v[-{ $i$ ,  $\Sigma_B$ }],
    metric[- $i$ , - $k$ ] v[ $k$ ] // toB // post
];]

dumpCV[v_] := Row@{
  v[ $i$ ], " = ", v[ $i$ ] // toB // MatrixForm // printNice, " ",
  v[- $i$ ], " = ", v[- $i$ ] // toB // MatrixForm // printNice
}
```

Specify components of a tensor  $T_{ij}$

```
allCV2[T_, T#, metric_, post_: (# &)] := Block[{},
  AllComponentValues[T[-{ $i$ ,  $\Sigma_B$ }, -{ $j$ ,  $\Sigma_B$ }], T# // post];
  AllComponentValues[T[{ $i$ ,  $\Sigma_B$ }, { $j$ ,  $\Sigma_B$ }],
    metric[ $i$ ,  $k$ ] metric[ $j$ ,  $l$ ] T[- $k$ , - $l$ ] // toB // post
];]
  AllComponentValues[T[{ $i$ ,  $\Sigma_B$ }, -{ $j$ ,  $\Sigma_B$ }],
    metric[ $i$ ,  $k$ ] T[- $k$ , - $j$ ] // toB // post
];]
  AllComponentValues[T[-{ $i$ ,  $\Sigma_B$ }, { $j$ ,  $\Sigma_B$ }],
    metric[ $j$ ,  $k$ ] T[- $i$ , - $k$ ] // toB // post
];]
```

```

dumpCV2[T_] := Row@{
  T[-i, -j], " = ", T[-i, -j] // toB // MatrixForm // printNice, " ",
  T[i, -j], " = ", T[i, -j] // toB // MatrixForm // printNice, " ",
  T[-i, j], " = ", T[-i, j] // toB // MatrixForm // printNice, " ",
  T[i, j], " = ", T[i, j] // toB // MatrixForm // printNice
}

```

Dump components of scalars, vectors, covectors and tensors

```

dumpScalar[h_ : (# &)] [X_] := Block[{e},
  e = X[] // toB // h;
  Print[e // printNice];
]

texScalar[h_ : (# &)] [X_] := Block[{e},
  e = X[] // toB // h;
  texOut[X == e]
]

dumpVector[h_ : (# &)] [v_] := Block[{e},
  e = v[i] // toB // h;
  Print[e // printNice];
]

texVector[h_ : (# &)] [v_] := Block[{e},
  e = v[i] // toB // h;
  texOut@# & /@ Thread[{v[r], v[θ], v[φ]} == e]
]

dumpCovector[h_ : (# &)] [v_] := Block[{e},
  e = v[-i] // toB // h;
  Print[e // printNice];
]

texCovector[h_ : (# &)] [v_] := Block[{e},
  e = v[-i] // toB // h;
  texOut@# & /@ Thread[{v[-r], v[-θ], v[-φ]} == e]
]

dumpOperator[h_ : (# &)] [T_] := Block[{e},
  e = T[i, -j] // toB // Diagonal // h;
  Print[e // printNice];
]

texOperator[h_ : (# &)] [T_] := Block[{e},
  e = T[i, -j] // toB // Diagonal // h;
  texOut@# & /@ Thread[{T[r, -r], T[θ, -θ], T[φ, -φ]} == e]
]

```

**defineField** -- Utility to define a scalar field

```

defineField[f_, printAs_, texAs_] := (
  fieldQ[f] ^= True;
  Tex[f] := texAs;
  xAct`xTensor`DefScalarFunction[f, PrintAs → printAs]
)

```



## UnderBar -- Operator to specify a scalar field

```
field = Sequence[ t[], r[] ];
UnderBar[ f_ ] := f[ t[], r[] ]
```

## $q, v, p, \lambda$ -- Scalar fields in the $h$ -sector

```
defineField[ hBeta, "q", "\\hShift" ]
defineField[ sLv, "v", "\\sLv" ]
defineField[ sLp, "p", "\\sLp" ]
defineField[ sLt, " $\lambda$ ", "\\sLt" ]
defineField[ sER, "R", "\\sER" ]
```

## $\alpha, \beta, A, B, K_1, K_2$ -- Scalar fields in the $g$ -sector

```
defineField[ gAlpha, " $\alpha$ ", "\\gAlpha" ]
defineField[ gBeta, " $\beta$ ", "\\gBeta" ]
defineField[ gEA, "A", "\\gEA" ]
defineField[ gEB, "B", "\\gEB" ]
defineField[ gKr, " $K_r$ ", "\\gK_{rr}" ]
defineField[ gK $\theta$ , " $K_\theta$ ", "\\gK_{\\theta\\theta}" ]
defineField[ gK1, " $K_1$ ", "\\gK_{1}" ]
defineField[ gK2, " $K_2$ ", "\\gK_{2}" ]
```

## $\tilde{\alpha}, \tilde{\beta}, \tilde{A}, \tilde{B}, \tilde{K}_1, \tilde{K}_2$ -- Scalar fields in the $f$ -sector

```
defineField[ fAlpha, " $\tilde{\alpha}$ ", "\\fAlpha" ]
defineField[ fBeta, " $\tilde{\beta}$ ", "\\fBeta" ]
defineField[ fEA, " $\tilde{A}$ ", "\\fEA" ]
defineField[ fEB, " $\tilde{B}$ ", "\\fEB" ]
defineField[ fKr, " $\tilde{K}_r$ ", "\\fK_{rr}" ]
defineField[ fK $\theta$ , " $\tilde{K}_\theta$ ", "\\fK_{\\theta\\theta}" ]
defineField[ fK1, " $\tilde{K}_1$ ", "\\fK_{1}" ]
defineField[ fK2, " $\tilde{K}_2$ ", "\\fK_{2}" ]
```

## Tensor components

### The spatial vielbeins $g_E, f_E$ and the metrics $\gamma_{ij}, \varphi_{ij}$

The Euclidean metric  $\hat{\delta}$ ,

```
sEta = IdentityMatrix[3];
```

The identity operator  $\hat{I}$ ,

```
sI = IdentityMatrix[3];
```

The spatial vielbein and the metric in the  $g$ -sector,

$$g_E = \begin{pmatrix} \underline{gEA} & 0 & 0 \\ 0 & \underline{gEB} & 0 \\ 0 & 0 & \underline{gEB} \sin[\theta] \end{pmatrix};$$

$$\gamma_{\mathbf{B}} = \begin{pmatrix} \frac{gEA^2}{A} & 0 & 0 \\ 0 & \frac{gEB^2}{B} & 0 \\ 0 & 0 & \frac{gEB^2}{B} \sin[\theta]^2 \end{pmatrix};$$

`MetricInBasis`[ $\gamma$ ,  $-\Sigma_B$ ,  $\gamma_{\mathbf{B}}$ ];

`MetricCompute`[ $\gamma$ ,  $\Sigma_B$ , `All`, `CVSimplify`  $\rightarrow$  `Simplify`]

The spatial vielbein and the metric in the  $f$ -sector,

$$fE_{\mathbf{B}} = \begin{pmatrix} \frac{fEA}{A} & 0 & 0 \\ 0 & \frac{fEB}{B} & 0 \\ 0 & 0 & \frac{fEB}{B} \sin[\theta] \end{pmatrix};$$

$$\varphi_{\mathbf{B}} = \begin{pmatrix} \frac{fEA^2}{A} & 0 & 0 \\ 0 & \frac{fEB^2}{B} & 0 \\ 0 & 0 & \frac{fEB^2}{B} \sin[\theta]^2 \end{pmatrix};$$

`MetricInBasis`[ $\varphi$ ,  $-\Sigma_B$ ,  $\varphi_{\mathbf{B}}$ ];

`MetricCompute`[ $\varphi$ ,  $\Sigma_B$ , `All`, `CVSimplify`  $\rightarrow$  `Simplify`]

Dump Cristoffel symbols,

`ChristoffelcdgPDEB`[ $i$ ,  $-j$ ,  $-k$ ] // `toB`;

`Join`[`{i, "r", "θ", "φ"}`],

`Join`[`{Flatten@Table`[ $\Gamma^i_{\text{coordToString}[j,k]}$ , `{j, 1, 3}`, `{k, 1, 3}`]]],

`Table`[

`Flatten@Table`[ $\%[[i, j, k]]$  // `printNice`, `{j, 1, 3}`, `{k, 1, 3}`],

`{i, 1, 3}]]` // `Transpose`] // `TableForm`

| $i$                       | $r$                                          | $\theta$                           | $\phi$                   |
|---------------------------|----------------------------------------------|------------------------------------|--------------------------|
| $\Gamma^i_{rr}$           | $\frac{\partial_r A}{A}$                     | 0                                  | 0                        |
| $\Gamma^i_{r\theta}$      | 0                                            | $\frac{\partial_r B}{B}$           | 0                        |
| $\Gamma^i_{r\phi}$        | 0                                            | 0                                  | $\frac{\partial_r B}{B}$ |
| $\Gamma^i_{\theta r}$     | 0                                            | $\frac{\partial_r B}{B}$           | 0                        |
| $\Gamma^i_{\theta\theta}$ | $-\frac{\partial_r B B}{A^2}$                | 0                                  | 0                        |
| $\Gamma^i_{\theta\phi}$   | 0                                            | 0                                  | $\text{Cot}[\theta]$     |
| $\Gamma^i_{\phi r}$       | 0                                            | 0                                  | $\frac{\partial_r B}{B}$ |
| $\Gamma^i_{\phi\theta}$   | 0                                            | 0                                  | $\text{Cot}[\theta]$     |
| $\Gamma^i_{\phi\phi}$     | $-\frac{\partial_r B \sin[\theta]^2 B}{A^2}$ | $-\text{Cos}[\theta] \sin[\theta]$ | 0                        |

`ChristoffelcdgPDEB`[ $i$ ,  $-j$ ,  $-k$ ] // `toB`;

`Row@Flatten@Riffle`[`Table`[`{`  
 $\Gamma^{\text{coordToString}[i]}_{jk}$ , " = ",

$\%[[i]]$  // `printNice` // `MatrixForm`

`}, {i, 1, 3}], ", "`]

$$\Gamma^r_{jk} = \begin{pmatrix} \frac{\partial_r A}{A} & 0 & 0 \\ 0 & -\frac{\partial_r B B}{A^2} & 0 \\ 0 & 0 & -\frac{\partial_r B \sin[\theta]^2 B}{A^2} \end{pmatrix}, \quad \Gamma^\theta_{jk} =$$

$$\begin{pmatrix} 0 & \frac{\partial_r B}{B} & 0 \\ \frac{\partial_r B}{B} & 0 & 0 \\ 0 & 0 & -\text{Cos}[\theta] \sin[\theta] \end{pmatrix}, \quad \Gamma^\phi_{jk} = \begin{pmatrix} 0 & 0 & \frac{\partial_r B}{B} \\ 0 & 0 & \text{Cot}[\theta] \\ \frac{\partial_r B}{B} & \text{Cot}[\theta] & 0 \end{pmatrix}$$

## The extrinsic curvatures $K_{ij}$ , $\tilde{K}_{ij}$

```

Quiet@DefTensor[gK[-i, -j],  $\Sigma$ t, PrintAs  $\rightarrow$  "K"]
Tex[gK] := "\\gK"

allCV2[gK,  $\left( \begin{array}{ccc} \underline{gKr} & 0 & 0 \\ 0 & \underline{gK\theta} & 0 \\ 0 & 0 & \underline{gK\theta} \sin[\theta[]]^2 \end{array} \right)$ ,  $\gamma$ ]

gKscalar[] = gK[k, -k] // toB // convert$K;
% // printNice

 $K_1 + 2 K_2$ 

Quiet@DefTensor[fK[-i, -j],  $\Sigma$ t, PrintAs  $\rightarrow$  " $\tilde{K}$ "]
Tex[fK] := "\\fK"

allCV2[fK,  $\left( \begin{array}{ccc} \underline{fKr} & 0 & 0 \\ 0 & \underline{fK\theta} & 0 \\ 0 & 0 & \underline{fK\theta} \sin[\theta[]]^2 \end{array} \right)$ ,  $\varphi$ ]

fKscalar[] = fK[k, -k] // toB // convert$K;
% // printNice

 $\tilde{K}_1 + 2 \tilde{K}_2$ 

```

## The shift vectors $\beta^i$ , $\tilde{\beta}^i$

```

eq$gBeta[t_, r_] := hBeta[t, r] + gAlpha[t, r] gEA[t, r]-1 sLv[t, r]
eq$fBeta[t_, r_] := hBeta[t, r] - fAlpha[t, r] fEA[t, r]-1 sLv[t, r]

instantiateBetas[e_] := Block[{gBeta, fBeta},
  gBeta[t_, r_] := eq$gBeta[t, r];
  fBeta[t_, r_] := eq$fBeta[t, r];
  e
]

Quiet@DefTensor[gBetaVec[i],  $\Sigma$ t, PrintAs  $\rightarrow$  " $\beta$ "]
Tex[gBetaVec] := "\\gShift"
allCV[gBetaVec, {gBeta, 0, 0},  $\gamma$ ]

Quiet@DefTensor[fBetaVec[i],  $\Sigma$ t, PrintAs  $\rightarrow$  " $\tilde{\beta}$ "]
Tex[fBetaVec] := "\\fShift"
allCV[fBetaVec, {fBeta, 0, 0},  $\varphi$ ];

```

# Projections of the Einstein and Ricci tensors

## Constraints

### The scalar constraints $C, \tilde{C}$

```
(RicciScalarcdg[] + gK[k, -k] gK[l, -l] - gK[-l, -j] gK[l, j]) / 2;
```

$$\text{gC\$scalar} = \% // \text{toB} // \text{convert\$K} // \text{FullSimplify} // \text{Expand};$$

```
%% == (% // printNice)
```

$$\frac{1}{2} \left( -K_{ij} K^{ij} + K^k_k K^\ell_\ell + R[D] \right) = \frac{1}{B^2} - \frac{(\partial_r B)^2}{A^2 B^2} + \frac{2 \partial_r A \partial_r B}{A^3 B} - \frac{2 \partial_r r B}{A^2 B} + 2 K_1 K_2 + K_2^2$$

```
(RicciScalarcdf[] + fK[k, -k] fK[l, -l] - fK[-l, -j] fK[l, j]) / 2;
```

$$\text{fC\$scalar} = \% // \text{toB} // \text{convert\$K} // \text{FullSimplify} // \text{Expand};$$

```
%% == (% // printNice)
```

$$\frac{1}{2} \left( -\tilde{K}_{ij} \tilde{K}^{ij} + \tilde{K}^k_k \tilde{K}^\ell_\ell + R[\tilde{D}] \right) = \frac{1}{\tilde{B}^2} - \frac{(\partial_r \tilde{B})^2}{\tilde{A}^2 \tilde{B}^2} + \frac{2 \partial_r \tilde{A} \partial_r \tilde{B}}{\tilde{A}^3 \tilde{B}} - \frac{2 \partial_r r \tilde{B}}{\tilde{A}^2 \tilde{B}} + 2 \tilde{K}_1 \tilde{K}_2 + \tilde{K}_2^2$$

### The vector constraints $C_i, \tilde{C}_i$ (note down indices!)

Note that we have index down below,

```
cdg[-j][gK[-i, j]] - \gamma[-i, j] cdg[-j][gK[k, -k]];
```

$$\text{gC\$vector} = \% // \text{toB} // \text{convert\$K} // \text{Expand};$$

```
%% == (% // printNice)
```

$$-(D_i K^k_k) + D_j K_i^j = \left\{ -2 \partial_r K_2 + \frac{2 \partial_r B K_1}{B} - \frac{2 \partial_r B K_2}{B}, 0, 0 \right\}$$

```
cdf[-j][fK[-i, j]] - \gamma[-i, j] cdf[-j][fK[k, -k]] (* \gamma[-i, j] = delta function! );
```

$$\text{fC\$vector} = \% // \text{toB} // \text{convert\$K} // \text{Expand};$$

```
%% == (% // printNice)
```

$$-(\tilde{D}_i \tilde{K}^k_k) + \tilde{D}_j \tilde{K}_i^j = \left\{ -2 \partial_r \tilde{K}_2 + \frac{2 \partial_r \tilde{B} \tilde{K}_1}{\tilde{B}} - \frac{2 \partial_r \tilde{B} \tilde{K}_2}{\tilde{B}}, 0, 0 \right\}$$

## Evolution equations

### The evolution eqs for the spatial metric of g

```
\gamma[-i, -j] // toB;
```

$$D[\#, t[]] \& / @ \%;$$

```
evol$dot$gSp = (% // Diagonal) / {2 gEA, 2 gEB, 2 gEB Sin[\theta[]]^2};
```

$$-2 gAlpha gK[-i, -j] + cdg[-i][gBetaVec[-j]] + cdg[-j][gBetaVec[-i]]$$

```
evol$eq$gSp = (% // toB // convert\$K // Diagonal) / {2 gEA, 2 gEB, 2 gEB Sin[\theta[]]^2};
```

$$-2 \alpha[t, r] K_{ij} + D_i \beta_j + D_j \beta_i$$

```
printHeader@"The evolution eqs for the spatial metric of g"
```

```
Print@printNice@# & /@ Thread[evol$dot$gSp == evol$eq$gSp];
```

The evolution eqs for the spatial metric of  $g$

$$\partial_t A = \partial_r \beta A + \partial_r A \beta - A \alpha K_1$$

$$\partial_t B = \partial_r B \beta - B \alpha K_2$$

$$\partial_t B = \partial_r B \beta - B \alpha K_2$$

## The evolution eqs for the spatial metric of f

```

φ[-i, -j] // toB;
D[#, t[]] & /@%;
evol$dot$fSp = (% // Diagonal) / {2 fEA, 2 fEB, 2 fEB Sin[θ[]]^2};

-2 fAlpha fK[-i, -j] + cdf[-i][fBetaVec[-j]] + cdf[-j][fBetaVec[-i]]
evol$eq$fSp = (% // toB // convert$K // Diagonal) / {2 fEA, 2 fEB, 2 fEB Sin[θ[]]^2};

-2 α[t, r] K̃i j + D̃i β̃j + D̃j β̃i

printHeader@"The evolution eqs for the spatial metric of f"
Print@printNice@# & /@ Thread[evol$dot$fSp == evol$eq$fSp];

```

The evolution eqs for the spatial metric of  $f$

$$\partial_t \tilde{A} = \partial_r \tilde{\beta} \tilde{A} + \partial_r \tilde{A} \tilde{\beta} - \tilde{A} \tilde{\alpha} \tilde{K}_1$$

$$\partial_t \tilde{B} = \partial_r \tilde{B} \tilde{\beta} - \tilde{B} \tilde{\alpha} \tilde{K}_2$$

$$\partial_t \tilde{B} = \partial_r \tilde{B} \tilde{\beta} - \tilde{B} \tilde{\alpha} \tilde{K}_2$$

## The evolution eqs for the extrinsic curvature of g

```

gK[-i, -j] // toB // convert$K;
D[#, t[]] & /@%;
rawEvol$dot$gK = (% // Diagonal) / {1, 1, Sin[θ[]]^2};

gAlpha (
  RicciCdG[-i, -j] - 2 gK[-i, -k] gK[k, -j] + gK[k, -k] gK[-i, -j]
) - cdg[-i][cdg[-j][gAlpha]] + Lied[gBetaVec[f], cdg][gK[-i, -j]]
rawEvol$eq$gK = (% // toB // convert$K // Diagonal // Simplify) / {1, 1, Sin[θ[]]^2};
evol$dot$gK = D[#, t[]] & /@ {gK1, gK2, gK2};
Thread[rawEvol$dot$gK == rawEvol$eq$gK] /.

Thread[evol$dot$gSp → evol$eq$gSp] // Simplify;
evol$eq$gK = {D[gK1, t[]] /. Solve[%[1], evol$dot$gK[[1]]][1, 1],
  D[gK2, t[]] /. Solve[%[2], evol$dot$gK[[2]]][1, 1],
  D[gK2, t[]] /. Solve[%[3], evol$dot$gK[[3]]][1, 1]} // Simplify // Expand;

α[t, r] (-2 Ki k Kkj + Ki j Kkk + R[D]i j) + Kk j (Di βk) +
  Ki k (Dj βk) + βk (Dk Ki j) + Γ[D, g]1i j α(0,1)[t, r] - ei1 ej1 α(0,2)[t, r]

printHeader@"The evolution eqs for the extrinsic curvature of g"
Print@printNice@# & /@ Thread[evol$dot$gK == evol$eq$gK];

```

The evolution eqs for the extrinsic curvature of  $g$

$$\partial_t K_1 = \frac{\partial_r A \partial_r \alpha}{A^3} - \frac{\partial_r r \alpha}{A^2} + \frac{2 \partial_r A \partial_r B \alpha}{A^3 B} - \frac{2 \partial_r r B \alpha}{A^2 B} + \partial_r K_1 \beta + \alpha K_1^2 + 2 \alpha K_1 K_2$$

$$\partial_t K_2 = -\frac{\partial_r B \partial_r \alpha}{A^2 B} + \frac{\alpha}{B^2} - \frac{(\partial_r B)^2 \alpha}{A^2 B^2} + \frac{\partial_r A \partial_r B \alpha}{A^3 B} - \frac{\partial_r r B \alpha}{A^2 B} + \partial_r K_2 \beta + \alpha K_1 K_2 + 2 \alpha K_2^2$$

$$\partial_t K_2 = -\frac{\partial_r B \partial_r \alpha}{A^2 B} + \frac{\alpha}{B^2} - \frac{(\partial_r B)^2 \alpha}{A^2 B^2} + \frac{\partial_r A \partial_r B \alpha}{A^3 B} - \frac{\partial_r r B \alpha}{A^2 B} + \partial_r K_2 \beta + \alpha K_1 K_2 + 2 \alpha K_2^2$$

## The evolution eqs for the extrinsic curvature of $f$

```

fK[-i, -j] // toB // convert$K;
D[#, t[]] & /@%;
rawEvol$dot$fK = (% // Diagonal) / {1, 1, Sin[Θ[]]^2};

fAlpha (
  Riccicdf[-i, -j] - 2 fK[-i, -k] fK[k, -j] + fK[k, -k] fK[-i, -j]
) - cdf[-i] [cdf[-j] [fAlpha] + Lied[fBetaVec[l], cdf] [fK[-i, -j]]
rawEvol$eq$fK = (% // toB // convert$K // Diagonal // Simplify) / {1, 1, Sin[Θ[]]^2};
evol$dot$fK = D[#, t[]] & /@ {fK1, fK2, fK2};
Thread[rawEvol$dot$fK == rawEvol$eq$fK] /.
  Thread[evol$dot$fSp → evol$eq$fSp] // Simplify;
evol$eq$fK = {D[fK1, t[]] /. Solve[%[[1]], evol$dot$fK[[1]]][1, 1],
  D[fK2, t[]] /. Solve[%[[2]], evol$dot$fK[[2]]][1, 1],
  D[fK2, t[]] /. Solve[%[[3]], evol$dot$fK[[3]]][1, 1]} // Simplify // Expand;

α[t, r] (-2  $\tilde{\kappa}_{ik} \tilde{\kappa}^k_j + \tilde{\kappa}_{ij} \tilde{\kappa}^k_k + R[\tilde{D}]_{ij}) + \tilde{\kappa}_{kj} (\tilde{D}_i \tilde{\beta}^k) +$ 
 $\tilde{\kappa}_{ik} (\tilde{D}_j \tilde{\beta}^k) + \tilde{\beta}^k (\tilde{D}_k \tilde{\kappa}_{ij}) + \Gamma[\tilde{D}, \mathcal{D}]^1_{ij} \tilde{\alpha}^{(0,1)}[t, r] - e_i^1 e_j^1 \tilde{\alpha}^{(0,2)}[t, r]$ 

printHeader@"The evolution eqs for the extrinsic curvature of  $f$ "
Print@printNice@# & /@ Thread[evol$dot$fK == evol$eq$fK];

```

---

The evolution eqs for the extrinsic curvature of  $f$

$$\begin{aligned}
 \partial_t \tilde{\kappa}_1 &= \frac{\partial_r \tilde{A} \partial_r \tilde{\alpha}}{\tilde{A}^3} - \frac{\partial_{rr} \tilde{\alpha}}{\tilde{A}^2} + \frac{2 \partial_r \tilde{A} \partial_r \tilde{B} \tilde{\alpha}}{\tilde{A}^3 \tilde{B}} - \frac{2 \partial_{rr} \tilde{B} \tilde{\alpha}}{\tilde{A}^2 \tilde{B}} + \partial_r \tilde{\kappa}_1 \tilde{\beta} + \tilde{\alpha} \tilde{\kappa}_1^2 + 2 \tilde{\alpha} \tilde{\kappa}_1 \tilde{\kappa}_2 \\
 \partial_t \tilde{\kappa}_2 &= -\frac{\partial_r \tilde{B} \partial_r \tilde{\alpha}}{\tilde{A}^2 \tilde{B}} + \frac{\tilde{\alpha}}{\tilde{B}^2} - \frac{(\partial_r \tilde{B})^2 \tilde{\alpha}}{\tilde{A}^2 \tilde{B}^2} + \frac{\partial_r \tilde{A} \partial_r \tilde{B} \tilde{\alpha}}{\tilde{A}^3 \tilde{B}} - \frac{\partial_{rr} \tilde{B} \tilde{\alpha}}{\tilde{A}^2 \tilde{B}} + \partial_r \tilde{\kappa}_2 \tilde{\beta} + \tilde{\alpha} \tilde{\kappa}_1 \tilde{\kappa}_2 + 2 \tilde{\alpha} \tilde{\kappa}_2^2 \\
 \partial_t \tilde{\kappa}_2 &= -\frac{\partial_r \tilde{B} \partial_r \tilde{\alpha}}{\tilde{A}^2 \tilde{B}} + \frac{\tilde{\alpha}}{\tilde{B}^2} - \frac{(\partial_r \tilde{B})^2 \tilde{\alpha}}{\tilde{A}^2 \tilde{B}^2} + \frac{\partial_r \tilde{A} \partial_r \tilde{B} \tilde{\alpha}}{\tilde{A}^3 \tilde{B}} - \frac{\partial_{rr} \tilde{B} \tilde{\alpha}}{\tilde{A}^2 \tilde{B}} + \partial_r \tilde{\kappa}_2 \tilde{\beta} + \tilde{\alpha} \tilde{\kappa}_1 \tilde{\kappa}_2 + 2 \tilde{\alpha} \tilde{\kappa}_2^2
 \end{aligned}$$

# Decomposition of the bimetric potential

## Definitions related to the potential

```
$Assumptions = sLt > 1;
```

### The beta parameters $\beta_n$

```
Quiet@DefInertHead[β]
Tex[β[n_]] := "\\beta_" <> Tex[n] <> " "
cdg[n_][β[m_]] := 0
cdf[n_][β[m_]] := 0
```

### The boost vectors and the Lorentz factor $v, p, \lambda, n, \tilde{n}$

```
sLp = { sLp, 0, 0 };
sLt = (1 + sLp^2)^{1/2};
sLv = sLp / sLt;

sgn = gE^{-1} . sLv;
Quiet@DefTensor[sgn[/_], Et, PrintAs -> "n"]
Tex[sgn] := "\\sgn"
allCV[sgn, Flatten@sgn, γ]

printHeader@"The boost vector n"
sgn // dumpVector[convert$p2λ]
```

The boost vector  $n$

```
{ p/Aλ, 0, 0 }

sfn = fE^{-1} . sLv;
Quiet@DefTensor[sfn[/_], Et, PrintAs -> "ñ"]
Tex[sfn] := "\\sfn"
allCV[sfn, Flatten@sfn, φ]

printHeader@"The boost vector ñ"
sfn // dumpVector[convert$p2λ]
```

The boost vector  $\tilde{n}$

```
{ p/λ Ñ, 0, 0 }
```

### The spatial part of the Lorentz transformation $Q, \tilde{Q}$

```
sLs = sI + 1/(1 + sLt) sLp . sLp^T // FullSimplify;

printHeader@"The spatial part of the Lorentz transformation Ñ"
Print@Row@{"Ñ =", sLs // printNice // MatrixForm}
```

The spatial part of the Lorentz transformation  $\tilde{\Lambda}$

$$\tilde{\Lambda} = \begin{pmatrix} \sqrt{1 + p^2} & 0 & 0 \\ 0 & 1 & 0 \\ 0 & 0 & 1 \end{pmatrix}$$

```

sgQ■ = gE■-1 · sLs■ · sLs■ · gE■;
sfQ■ = fE■-1 · sLs■ · sLs■ · fE■;

printHeader@"The transformed LT spatial part Q and Q̃"
Print@
  Row@{"Q =" , sgQ■ // printNice // MatrixForm, " , Q̃ = " , sfQ■ // printNice // MatrixForm}

```

The transformed LT spatial part  $Q$  and  $\tilde{Q}$

$$Q = \begin{pmatrix} 1 + \textcolor{green}{p}^2 & 0 & 0 \\ 0 & 1 & 0 \\ 0 & 0 & 1 \end{pmatrix}, \quad \tilde{Q} = \begin{pmatrix} 1 + \textcolor{green}{p}^2 & 0 & 0 \\ 0 & 1 & 0 \\ 0 & 0 & 1 \end{pmatrix}$$

## The spatial square-root variables: $\mathcal{D}$ , $\mathcal{B}$ , $\tilde{\mathcal{D}}$ , $\tilde{\mathcal{B}}$ , $\mathcal{V}$ , $\tilde{\mathcal{V}}$ , $\mathcal{U}$ , $\tilde{\mathcal{U}}$

$\mathcal{D}, \mathcal{B}$

```

sgD■ = fE■-1 · sLs■-1 · gE■;
Quiet@DefTensor[sgD[-i, -j], Σt, PrintAs → "D"]
Tex[sgD] := "\\sgD"
allCV2[sgD, γ■ · sgD■ // Simplify, γ]

printHeader@"The spatial square root variable D"
sgD // dumpOperator[convert$p2λ]

```

The spatial square root variable  $\mathcal{D}$

$$\left\{ \frac{\textcolor{blue}{A}}{\textcolor{green}{λ} \tilde{\textcolor{red}{A}}}, \frac{\textcolor{blue}{B}}{\tilde{\textcolor{red}{B}}}, \frac{\textcolor{blue}{B}}{\tilde{\textcolor{red}{B}}} \right\}$$

```

sgB■ = gE■-1 · sLs■ · fE■;
Quiet@DefTensor[sgB[-i, -j], Σt, PrintAs → "B"]
Tex[sgB] := "\\sgB"
allCV2[sgB, γ■ · sgB■ // Simplify, γ]

printHeader@"The spatial square root variable B"
sgB // dumpOperator[convert$p2λ]

```

The spatial square root variable  $\mathcal{B}$

$$\left\{ \frac{\textcolor{green}{λ} \tilde{\textcolor{red}{A}}}{\textcolor{blue}{A}}, \frac{\tilde{\textcolor{red}{B}}}{\textcolor{blue}{B}}, \frac{\tilde{\textcolor{red}{B}}}{\textcolor{blue}{B}} \right\}$$

$\tilde{\mathcal{D}}, \tilde{\mathcal{B}}$

```

sfD■ = gE■-1 · sLs■-1 · fE■;
Quiet@DefTensor[sfD[-i, -j], Σt, PrintAs → "D̃"]
Tex[sfD] := "\\sfD"
allCV2[sfD, φ■ · sfD■ // Simplify, φ]

printHeader@"The spatial square root variable D̃"
sfD // dumpOperator[convert$p2λ]

```

The spatial square root variable  $\tilde{\mathcal{D}}$

$$\left\{ \frac{\tilde{\textcolor{red}{A}}}{\textcolor{blue}{A} \textcolor{green}{λ}}, \frac{\tilde{\textcolor{red}{B}}}{\textcolor{blue}{B}}, \frac{\tilde{\textcolor{red}{B}}}{\textcolor{blue}{B}} \right\}$$



```

sfB = fE-1 · sLs · gE;
Quiet@DefTensor[sfB[-i, -j], {t, PrintAs → "B"}]
Tex[sfB] := "\\sfB"
allCV2[sfB, ϕ · sfB // Simplify, ϕ]

printHeader@"The spatial square root variable  $\tilde{B}$ "
sfB // dumpOperator[convert$2λ]

```

The spatial square root variable  $\tilde{B}$

$$\left\{ \frac{A\lambda}{\tilde{A}}, \frac{B}{\tilde{B}}, \frac{B}{\tilde{B}} \right\}$$

```

sgB = Inverse@sgD ∧ sgB = sfD · sfQ ∧
sfB = Inverse@sfD ∧ sfB = sgD · sfQ // Simplify // Framed

```

True

$\mathcal{V}, \tilde{\mathcal{V}}$

```

sgVn := εn[sfD]
sgV[] = (Vsign ∑n=04 β[n] sgVn) // simplifyShiftedESP // convert$2λ;
Tex[sgV] := "\\sgV"

printHeader@"The variable  $\mathcal{V}$ "
sgV // dumpScalar[]

```

The variable  $\mathcal{V}$

$$\langle R \rangle_0^2 + \frac{\langle R \rangle_1^2 \tilde{A}}{A\lambda}$$

```

sfVn := sLt-1 εn-1[sgB]
sfV[] = (Vsign ∑n=04 β[n] sfVn) // simplifyShiftedESP // convert$2λ;
Tex[sfV] := "\\sfV"

printHeader@"The variable  $\tilde{\mathcal{V}}$ "
sfV // dumpScalar[]

```

The variable  $\tilde{\mathcal{V}}$

$$\frac{\langle R \rangle_1^2}{\lambda} + \frac{\langle R \rangle_2^2 \tilde{A}}{A}$$

$\mathcal{U}, \tilde{\mathcal{U}}$

```

sgUn := sLt-1 Yn-1[sgB]
sgU[] = (Vsign ∑n=04 β[n] sgUn);
Quiet@DefTensor[sgU[-i, -j], {t, PrintAs → "U"}]
Tex[sgU] := "\\sgU"
allCV2[sgU, γ · sgU // Simplify, γ]

printHeader@"The variable  $\mathcal{U}$ "
sgU // dumpOperator[convert$2λ@simplifyShiftedESP@# &]

```

The variable  $\mathcal{U}$

```


$$\left\{ \frac{\langle R \rangle_1^2}{\lambda}, \frac{\langle R \rangle_1^1}{\lambda} + \frac{\langle R \rangle_2^1 \tilde{A}}{A}, \frac{\langle R \rangle_1^1}{\lambda} + \frac{\langle R \rangle_2^1 \tilde{A}}{A} \right\}$$


sfUn := sfDn · Yn-1[sfDn]
sfU =  $\left( \$Vsign \sum_{n=0}^4 \beta[n] \text{sfU}_n \right);$ 

Quiet@DefTensor[sfU[-i, -j],  $\Sigma$ t, PrintAs → "Ũ"]
Tex[sfU] := "\\sfU"
allCV2[sfU, ϕn · sfUn // Simplify, ϕ]

printHeader@"The variable Ũ"
sfU // dumpOperator[convert$2λ@simplifyShiftedESP@# &]

```

The variable Ũ

$$\left\{ \frac{\langle R \rangle_1^2 \tilde{A}}{A \lambda}, R \left( \langle R \rangle_1^1 + \frac{\langle R \rangle_2^1 \tilde{A}}{A \lambda} \right), R \left( \langle R \rangle_1^1 + \frac{\langle R \rangle_2^1 \tilde{A}}{A \lambda} \right) \right\}$$

(Q<sub>Ũ</sub>), (Q̃<sub>Ũ</sub>)

```

sgQUn := sgBn · Yn-1[sfDn]
sgQU =  $\left( \$Vsign \sum_{n=0}^4 \beta[n] \text{sgQU}_n \right);$ 

Quiet@DefTensor[sgQU[-i, -j],  $\Sigma$ t, PrintAs → "Q̃Ũ"]
Tex[sgQU] := "\\sgQU"
allCV2[sgQU, γn · sgQUn // Simplify, γ]

printHeader@"The variable (Q̃Ũ)"
sgQU // dumpOperator[convert$2λ@simplifyShiftedESP@# &]

```

The variable (QŨ)

$$\left\{ \frac{\langle R \rangle_1^2 \lambda \tilde{A}}{A}, R \left( \langle R \rangle_1^1 + \frac{\langle R \rangle_2^1 \tilde{A}}{A \lambda} \right), R \left( \langle R \rangle_1^1 + \frac{\langle R \rangle_2^1 \tilde{A}}{A \lambda} \right) \right\}$$

```

sfQUn := sLtn-1 sfQn · Yn-1[sgBn]
sfQU =  $\left( \$Vsign \sum_{n=0}^4 \beta[n] \text{sfQU}_n \right);$ 

Quiet@DefTensor[sfQU[-i, -j],  $\Sigma$ t, PrintAs → "Q̃Ũ"]
Tex[sfQU] := "\\sfQU"
allCV2[sfQU, ϕn · sfQUn // Simplify, ϕ]

printHeader@"The variable (Q̃Ũ)"
sfQU // dumpOperator[convert$2λ@simplifyShiftedESP@# &]

```

The variable (Q̃Ũ)

$$\left\{ \langle R \rangle_1^2 \lambda, \frac{\langle R \rangle_1^1}{\lambda} + \frac{\langle R \rangle_2^1 \tilde{A}}{A}, \frac{\langle R \rangle_1^1}{\lambda} + \frac{\langle R \rangle_2^1 \tilde{A}}{A} \right\}$$

## Projections of V<sub>g</sub> and V<sub>f</sub>

ρ, ρ̃ -----The normal projection of V<sub>gf</sub>

```

gρn := -εn[sgBn]
gρ[] =  $\left( \$Vsign \sum_{n=0}^4 \beta[n] g\rho_n \right) // \text{simplifyShiftedESP} // \text{convert\$2}\lambda;$ 
Tex[gρ] := "\\grho"

```

```
printHeader@"The projection  $\rho[V_g]$ "
gp // dumpScalar[]
```

The projection  $\rho[V_g]$

$$-\langle R \rangle_0^2 - \frac{\langle R \rangle_1^2 \lambda \tilde{A}}{A}$$

```
fpn := -sLt  $\epsilon_{n-1}$  [sfD] Det@gE / Det@fE
```

```
fp[] =  $\left( \$Vsign \sum_{n=0}^4 \beta[n] fp_n \right)$  // simplifyShiftedESP // convert$2λ // Expand;
```

```
Tex[fp] := "\frho"
```

```
printHeader@"The projection  $\rho[V_f]$ "
```

```
fp // dumpScalar[Expand]
```

The projection  $\rho[V_f]$

$$-\frac{\langle R \rangle_2^2}{R^2} - \frac{\langle R \rangle_1^2 A \lambda}{R^2 \tilde{A}}$$

$j_i$  ----- The mixed projection of  $V_g$

```
gjn := -sgQUn · sgn
```

```
gj[] =  $\left( \$Vsign \sum_{n=0}^4 \beta[n] gj_n \right)$  // simplifyShiftedESP;
```

```
Quiet@DefTensor[gj[/],  $\Sigma t$ , PrintAs → "j"]
```

```
Tex[gj] := "\gjota"
```

```
allCV[gj, Flatten@gj[],  $\gamma$ ]
```

```
printHeader@"The projection  $j_r[V_g]$ "
```

```
gj // dumpCovector[]
```

The projection  $j_r[V_g]$

$$\{-\langle R \rangle_1^2 p \tilde{A}, 0, 0\}$$

Verify the identity:  $\rho + \mathcal{V} = n^k j_k$ ,  $e_n(\tilde{B}) - e_n(\tilde{D}) = Q \tilde{\mathcal{U}}.n$ ,  $[-e_n(\tilde{B})] + [e_n(\tilde{D})] = [-Q \tilde{\mathcal{U}}.n]$ ,

```
gp[] + sgV[] == (sgn[/] gj[-/] // toB) // Simplify // convert$2λ // Framed
```

True

$J^i_j, \tilde{J}^i_j$  ----- The full spatial projections of  $V_{gf}$

```
gJn := sgVn sI - sgQUn + fAlpha gAlpha-1 sgUn
```

```
gJ[] =  $\left( \$Vsign \sum_{n=0}^4 \beta[n] gJ_n \right)$  // simplifyShiftedESP;
```

```
Quiet@DefTensor[gJ[-/, -/],  $\Sigma t$ , PrintAs → "J"]
```

```
Tex[gJ] := "\gJota"
```

```
allCV2[gJ,  $\gamma$  · gJ[],  $\gamma$ ]
```

```
printHeader@"The projection J[Vg]"
```

```
gJ // dumpOperator[Expand@convert$2λ@# &]
```

The projection J[V<sub>g</sub>]

$$\left\{ \langle R \rangle_0^2 + \frac{\langle R \rangle_1^2 \tilde{A}}{A \lambda} - \frac{\langle R \rangle_1^2 \lambda \tilde{A}}{A} + \frac{\langle R \rangle_1^2 \tilde{\alpha}}{\alpha \lambda}, \langle R \rangle_0^1 + \frac{\langle R \rangle_1^1 \tilde{A}}{A \lambda} + \frac{\langle R \rangle_1^1 \tilde{\alpha}}{\alpha \lambda} + \frac{\langle R \rangle_2^1 \tilde{A} \tilde{\alpha}}{A \alpha}, \langle R \rangle_0^1 + \frac{\langle R \rangle_1^1 \tilde{A}}{A \lambda} + \frac{\langle R \rangle_1^1 \tilde{\alpha}}{\alpha \lambda} + \frac{\langle R \rangle_2^1 \tilde{A} \tilde{\alpha}}{A \alpha} \right\}$$

```

fJn := (sfVn sIn - sfQUn + gAlpha fAlpha-1 sfUn) Det@gEn / Det@fEn
fJn = (Vsign ∑n=04 β[n] fJn) // simplifyShiftedESP;
Quiet@DefTensor[fJ[-i, -j], St, PrintAs → "J̃"]
Tex[fJ] := "\\fJota"
allCV2[fJ, φn · fJn, φ]

printHeader@"The projection J[Vf]"
fJ // dumpOperator[Expand@convert$p2λ@# &]

```

The projection J[V<sub>f</sub>]

$$\left\{ \frac{\langle R \rangle_2^2}{R^2} + \frac{\langle R \rangle_1^2 A}{R^2 \lambda \tilde{A}} - \frac{\langle R \rangle_1^2 A \lambda}{R^2 \tilde{A}} + \frac{\langle R \rangle_1^2 \alpha}{R^2 \lambda \tilde{\alpha}}, \frac{\langle R \rangle_3}{R} + \frac{\langle R \rangle_2^{\frac{1}{2}} A}{R \lambda \tilde{A}} + \frac{\langle R \rangle_2^{\frac{1}{2}} \alpha}{R \lambda \tilde{\alpha}} + \frac{\langle R \rangle_1^{\frac{1}{2}} A \alpha}{R \tilde{A} \tilde{\alpha}}, \frac{\langle R \rangle_3}{R} + \frac{\langle R \rangle_2^{\frac{1}{2}} A}{R \lambda \tilde{A}} + \frac{\langle R \rangle_2^{\frac{1}{2}} \alpha}{R \lambda \tilde{\alpha}} + \frac{\langle R \rangle_1^{\frac{1}{2}} A \alpha}{R \tilde{A} \tilde{\alpha}} \right\}$$

$J_j^i - \frac{1}{2} \delta_j^i (J - \rho)$  ----- The contributions to EoM

```

gJρ = (gJ[i, -j] - 1/2 γ[i, -j] (gJ[k, -k] - XX) // toB) /. XX -> gρ[] // Diagonal // convert$p2λ;

printHeader@"The g EoM contribution J̃ij - 1/2 δij (J - ρ)"
Print@printNice@# & /@ gJρ;

```

The g EoM contribution  $J_j^i - \frac{1}{2} \delta_j^i (J - \rho)$

$$\begin{aligned}
& -\frac{1}{2 A \alpha \lambda} \left( 2 \langle R \rangle_1^2 \alpha \lambda^2 \tilde{A} + (2 \langle R \rangle_1^{\frac{1}{2}} - \langle R \rangle_1^2) (\alpha \tilde{A} + A \tilde{\alpha}) + 2 \lambda (\langle R \rangle_0^{\frac{1}{2}} A \alpha + \langle R \rangle_2^{\frac{1}{2}} \tilde{A} \tilde{\alpha}) \right) \\
& - \langle R \rangle_0^2 - \frac{\langle R \rangle_1^2 (\alpha \tilde{A} + A \tilde{\alpha})}{2 A \alpha \lambda} \\
& - \langle R \rangle_0^2 - \frac{\langle R \rangle_1^2 (\alpha \tilde{A} + A \tilde{\alpha})}{2 A \alpha \lambda}
\end{aligned}$$

```

fJρ = (fJ[i, -j] - 1/2 γ[i, -j] (fJ[k, -k] - XX) // toB) /. XX -> fρ[] // Diagonal // convert$p2λ;

printHeader@"The f EoM contribution J̃ij - 1/2 δij (J - ρ)"
Print@printNice@# & /@ fJρ;

```

The f EoM contribution  $J_j^i - \frac{1}{2} \delta_j^i (J - \rho)$

$$\begin{aligned}
& \frac{1}{2 R^2 \lambda \tilde{A} \tilde{\alpha}} \left( -2 \langle R \rangle_1^2 A \lambda^2 \tilde{\alpha} + (\langle R \rangle_1^2 - 2 \langle R \rangle_2^{\frac{1}{2}} R) (\alpha \tilde{A} + A \tilde{\alpha}) - 2 R \lambda (\langle R \rangle_1^{\frac{1}{2}} A \alpha + \langle R \rangle_3^{\frac{1}{2}} \tilde{A} \tilde{\alpha}) \right) \\
& - \frac{2 \langle R \rangle_2^2 + \frac{\langle R \rangle_1^2 (\alpha \tilde{A} + A \tilde{\alpha})}{\lambda \tilde{A} \tilde{\alpha}}}{2 R^2} \\
& - \frac{2 \langle R \rangle_2^2 + \frac{\langle R \rangle_1^2 (\alpha \tilde{A} + A \tilde{\alpha})}{\lambda \tilde{A} \tilde{\alpha}}}{2 R^2}
\end{aligned}$$

# The bimetric conservation law

$$u_j^i \left( D_i n^j - K^j_i \right) + \tilde{u}_j^i \left( \tilde{D}_i \tilde{n}^j + \tilde{K}^j_i \right) - D_i [u_j^i n^j] = 0.$$

```

CC0Ag = -sgU[i, -j] gK[j, -i];
CC0Af = sfU[i, -j] fK[j, -i];
CC0B = sgU[i, -j] cdg[-i][sgn[j]] + sfU[i, -j] cdf[-i][sfn[j]] - cdg[-i][sgU[i, -j] sgn[j]];
CC0Ag + CC0Af + CC0B // printNice


$$\tilde{K}^j_i \tilde{u}^i_j - K^j_i u^i_j + \tilde{u}^i_j \left( \tilde{D}_i \tilde{n}^j \right) - n^j \left( D_i u^i_j \right)$$


CC1Ag = CC0Ag // toB // convert$K // convert$p2λ;
CC1Af = CC0Af // toB // convert$K // convert$p2λ;
CC1B = CC0B // toB // convert$K // convert$p2λ;

CC2Ag = sLt gEA CC1Ag // simplifyShiftedESP;
% // printNice


$$-2 \langle R \rangle_2^{\frac{1}{2}} \lambda \tilde{A} K_2 - A \left( \langle R \rangle_1^2 K_1 + 2 \langle R \rangle_1^{\frac{1}{2}} K_2 \right)$$


CC2Af = sLt gEA CC1Af // simplifyShiftedESP;
% // printNice


$$2 \langle R \rangle_1^{\frac{1}{2}} A R \lambda \tilde{K}_2 + \tilde{A} \left( -2 \langle R \rangle_1^{\frac{1}{2}} \tilde{K}_2 + \langle R \rangle_1^2 \left( \tilde{K}_1 + 2 \tilde{K}_2 \right) \right)$$


CC2B = sLt gEA CC1B // simplifyShiftedESP;
% // printNice


$$\frac{\partial_r p \langle R \rangle_1^2}{\lambda} + \frac{2 \partial_r \tilde{B} \langle R \rangle_1^{\frac{1}{2}} A p}{B \tilde{A}} + \frac{2 \partial_r B \langle R \rangle_2^{\frac{1}{2}} p \tilde{A}}{A B}$$


CC2Ag + CC2Af // Expand // Collect[#, {sLp, gEA, fEA}, Simplify] &;
% // printNice

If[Head@%% === Plus, Print@printNice@# & /@%%];


$$\tilde{A} \left( -2 \langle R \rangle_2^{\frac{1}{2}} \lambda K_2 + \langle R \rangle_1^2 \tilde{K}_1 - 2 \left( \langle R \rangle_1^{\frac{1}{2}} - \langle R \rangle_1^2 \right) \tilde{K}_2 \right) + A \left( -\langle R \rangle_1^2 K_1 - 2 \langle R \rangle_1^{\frac{1}{2}} K_2 + 2 \langle R \rangle_1^{\frac{1}{2}} R \lambda \tilde{K}_2 \right)$$



$$\tilde{A} \left( -2 \langle R \rangle_2^{\frac{1}{2}} \lambda K_2 + \langle R \rangle_1^2 \tilde{K}_1 - 2 \left( \langle R \rangle_1^{\frac{1}{2}} - \langle R \rangle_1^2 \right) \tilde{K}_2 \right)$$



$$A \left( -\langle R \rangle_1^2 K_1 - 2 \langle R \rangle_1^{\frac{1}{2}} K_2 + 2 \langle R \rangle_1^{\frac{1}{2}} R \lambda \tilde{K}_2 \right)$$


CC2B // Expand // Collect[#, {sLp, gEA, fEA}, Simplify] &;
% // printNice

If[Head@%% === Plus, Print@printNice@# & /@%%];


$$\frac{\partial_r p \langle R \rangle_1^2}{\lambda} + p \left( \frac{2 \partial_r \tilde{B} \langle R \rangle_1^{\frac{1}{2}} A}{B \tilde{A}} + \frac{2 \partial_r B \langle R \rangle_2^{\frac{1}{2}} \tilde{A}}{A B} \right)$$



$$p \left( \frac{2 \partial_r \tilde{B} \langle R \rangle_1^{\frac{1}{2}} A}{B \tilde{A}} + \frac{2 \partial_r B \langle R \rangle_2^{\frac{1}{2}} \tilde{A}}{A B} \right)$$



$$\frac{\partial_r p \langle R \rangle_1^2}{\lambda}$$


eq$bimConsLaw = CC2Ag + CC2Af + CC2B // simplifyShiftedESP;
printHeader@"The bimetric conservation law"
eq$bimConsLaw // printNice // Print

```

$$\frac{\partial_{\mathbf{r}} \mathbf{p} \langle \mathbf{R} \rangle_1^2}{\lambda} + \frac{2 \partial_{\mathbf{r}} \tilde{\mathbf{B}} \langle \mathbf{R} \rangle_1^1 \mathbf{A} \mathbf{p}}{\mathbf{B} \tilde{\mathbf{A}}} +$$

$$\tilde{\mathbf{A}} \left( 2 \langle \mathbf{R} \rangle_2^1 \left( \frac{\partial_{\mathbf{r}} \mathbf{B} \mathbf{p}}{\mathbf{A} \mathbf{B}} - \lambda \mathbf{K}_2 \right) + \langle \mathbf{R} \rangle_1^2 \tilde{\mathbf{K}}_1 + 2 \left( -\langle \mathbf{R} \rangle_1^1 + \langle \mathbf{R} \rangle_1^2 \right) \tilde{\mathbf{K}}_2 \right) - \mathbf{A} \left( \langle \mathbf{R} \rangle_1^2 \mathbf{K}_1 + 2 \langle \mathbf{R} \rangle_1^1 \left( \mathbf{K}_2 - \mathbf{R} \lambda \tilde{\mathbf{K}}_2 \right) \right)$$

**Note down indices for  $j_r$  !**

```
gj[{1, -ΣB}];
% == (% // toB) // printNice
j_1 == -⟨R⟩_1^2 p Ã
```

**NOTE: The solution below is for vacuum!**

```
sLp;
solved$p = % /. Solve[gj[{1, -ΣB}] == gC$vector[[1]] // toB, sLp][[1, 1]];
Row@{printNice@(% == ""), (printNice@%)}
p == - \frac{2 \left( -\partial_{\mathbf{r}} \mathbf{K}_2 \mathbf{B} + \partial_{\mathbf{r}} \mathbf{B} \mathbf{K}_1 - \partial_{\mathbf{r}} \mathbf{B} \mathbf{K}_2 \right)}{\langle \mathbf{R} \rangle_1^2 \mathbf{B} \tilde{\mathbf{A}}}
```

## Save the module “bimetric-ss-nr.m”

Note: `evol$P` is calculated in the ‘verification’ notebook!

```
evol$P := (2 * fAlpha[t[], r[]] * P[1, 2, sER[t[], r[]]] *
  (gEA[t[], r[]] * sLt[t[], r[]] * Derivative[0, 1][fEB][t[], r[]] -
    fEA[t[], r[]] * Derivative[0, 1][gEB][t[], r[]]) +
  P[1, 1, sER[t[], r[]]] * (-2 * fAlpha[t[], r[]] * fEA[t[], r[]] *
    fK2[t[], r[]] * gEA[t[], r[]] * gEB[t[], r[]] * sLp[t[], r[]] +
    2 * gAlpha[t[], r[]] * (gEA[t[], r[]] * Derivative[0, 1][fEB][t[], r[]] +
      fEA[t[], r[]] * (gEA[t[], r[]] * gEB[t[], r[]] * gK2[t[], r[]] * sLp[t[], r[]] -
        sLt[t[], r[]] * Derivative[0, 1][gEB][t[], r[]]))) +
  gEB[t[], r[]] * P[2, 1, sER[t[], r[]]] * (fAlpha[t[], r[]] * fEA[t[], r[]] *
    (fK1[t[], r[]] + 2 * fK2[t[], r[]]) * gEA[t[], r[]] * sLp[t[], r[]] +
    gEA[t[], r[]] * sLt[t[], r[]] * Derivative[0, 1][fAlpha][t[], r[]] +
    fEA[t[], r[]] * (gAlpha[t[], r[]] * gEA[t[], r[]] * gK1[t[], r[]] * sLp[t[], r[]] -
      sLt[t[], r[]] * Derivative[0, 1][gAlpha][t[], r[]] +
      gEA[t[], r[]] * hBeta[t[], r[]] * Derivative[0, 1][sLp][t[], r[]])) /
  (fEA[t[], r[]] * gEA[t[], r[]] * gEB[t[], r[]] * P[2, 1, sER[t[], r[]]])
```

The regularized version (where  $f$  is replaced by  $fr$ ).

```
regularizeTimeDerivative[f_, evol_] := D[f, t[]] /. Solve[D[f r[], t[]] == evol, D[f, t[]]] [[1]];
regularEvolB[f_, evol_] := If[$regularB, regularizeTimeDerivative[f, evol], evol]
regularEvolB[B, evol$eq$gSp[[2]]] // printNice;

appendDefs[name_, expr_] := (defs = defs <> name <> "[t_, r_] := " <>
  ToString@InputForm[
    Block[{gEB, fEB},
      If[$regularB,
        gEB[t_, r_] := gB[t, r] r;
        fEB[t_, r_] := fB[t, r] r,
        gEB[t_, r_] := gB[t, r];
        fEB[t_, r_] := fB[t, r]
      ];
      expr /. {
        t[] → t, r[] → r, gEA → gA, fEA → fA,
        gAlpha → gAlp, gBeta → gBet, fAlpha → fAlp, fBeta → fBet, sER → R,
        sLp → p, sLv → v, sLt → Lt, hBeta → q
      } // If[$regularB, # // Simplify, #] &
    ] <> "\n\n";)
```

```

exportDefs[] := Block[
{
  prefix = If[$regularB, "eqr$", "eqn$"],
  evolPrefix = If[$regularB, "evol$eqr$", "evol$eqn$"]
},
If[$regularB,
  defs = defs <> "(* Usual gB and fB *)" <> "\n\n",
  defs = defs <> "(* Regularized gB and fB *)" <> "\n\n",
];
defs = defs <> "(* Shift vectors *)" <> "\n\n";
appendDefs[prefix <> "gBet", eq$gBeta];
appendDefs[prefix <> "fBet", eq$fBeta];
defs = defs <>
  "(* Projections of the bimeric stress-energy tensor in the g-sector *)" <> "\n\n";
appendDefs[prefix <> "gV$\rho", g\rho[]];
appendDefs[prefix <> "gV$j", toB[gj[-/]] [1]];
appendDefs[prefix <> "gV$JK1", gJ\rho [1]]; (* Contributions of J & \rho into EoM *)
appendDefs[prefix <> "gV$JK2", gJ\rho [2]];
defs = defs <>
  "(* Projections of the bimeric stress-energy tensor in the g-sector *)" <> "\n\n";
appendDefs[prefix <> "fV$\rho", f\rho[]];
appendDefs[prefix <> "fV$j", -toB[gj[-/]] [1] * Det@gE / Det@fE];
appendDefs[prefix <> "fV$JK1", fJ\rho [1]]; (* Contributions of J & \rho into EoM *)
appendDefs[prefix <> "fV$JK2", fJ\rho [2]];
defs = defs <> "(* Scalar constraints *)" <> "\n\n";
appendDefs[prefix <> "gC$\rho", gC$scalar];
appendDefs[prefix <> "fC$\rho", fC$scalar];
defs = defs <> "(* Vector constraints *)" <> "\n\n";
appendDefs[prefix <> "gC$j", gC$vector [1]];
appendDefs[prefix <> "fC$j", fC$vector [1]];
defs = defs <> "(* The solved p and its time evolution *)" <> "\n\n";
appendDefs[prefix <> "p", solved$p];
appendDefs[evolPrefix <> "p", evol$p];
defs = defs <> "(* Bimetric conservation law *)" <> "\n\n";
appendDefs[prefix <> "bimConsLaw", eq$bimConsLaw];
defs =
  defs <> "(* Evolution equations in the g-Sector (including sources) *)" <> "\n\n";
appendDefs[evolPrefix <> "gA", evol$eq$gSp [1]];
appendDefs[evolPrefix <> "gB", regularEvolB[gB, evol$eq$gSp [2]]];
appendDefs[evolPrefix <> "gK1", evol$eq$gK [1] - k$g gAlpha g$JK1];
appendDefs[evolPrefix <> "gK2", evol$eq$gK [2] - k$g gAlpha g$JK2];
defs =
  defs <> "(* Evolution equations in the f-Sector (including sources) *)" <> "\n\n";
appendDefs[evolPrefix <> "fA", evol$eq$fSp [1]];
appendDefs[evolPrefix <> "fB", regularEvolB[fB, evol$eq$fSp [2]]];
appendDefs[evolPrefix <> "fK1", evol$eq$fK [1] - k$f fAlpha f$JK1];
appendDefs[evolPrefix <> "fK2", evol$eq$fK [2] - k$f fAlpha f$JK2];
]

```



```

useEqn$[] := Block[{ },
  eq$gBet = eqn$gBet; eq$fBet = eqn$fBet;
  eq$gV$p = eqn$gV$p; eq$gV$j = eqn$gV$j;
  eq$gV$JK1 = eqn$gV$JK1; eq$gV$JK2 = eqn$gV$JK2;
  eq$fV$p = eqn$fV$p; eq$fV$j = eqn$fV$j;
  eq$fV$JK1 = eqn$fV$JK1; eq$fV$JK2 = eqn$fV$JK2;
  eq$gC$p = eqn$gC$p; eq$fC$p = eqn$fC$p;
  eq$gC$j = eqn$gC$j; eq$fC$j = eqn$fC$j;
  eq$p = eqn$p; evol$eq$p = evol$eqn$p;
  eq$bimConsLaw = eqn$bimConsLaw;
  evol$eq$gA = evol$eqn$gA; evol$eq$gB = evol$eqn$gB;
  evol$eq$gK1 = evol$eqn$gK1; evol$eq$gK2 = evol$eqn$gK2;
  evol$eq$fA = evol$eqn$fA; evol$eq$fB = evol$eqn$fB;
  evol$eq$fK1 = evol$eqn$fK1; evol$eq$fK2 = evol$eqn$fK2;
  eq$gW = eqn$gW; eq$fW = eqn$fW; eq$cW = eqn$cW;
]

useEqr$[] := Block[{ },
  eq$gBet = eqr$gBet; eq$fBet = eqr$fBet;
  eq$gV$p = eqr$gV$p; eq$gV$j = eqr$gV$j;
  eq$gV$JK1 = eqr$gV$JK1; eq$gV$JK2 = eqr$gV$JK2;
  eq$fV$p = eqr$fV$p; eq$fV$j = eqr$fV$j;
  eq$fV$JK1 = eqr$fV$JK1; eq$fV$JK2 = eqr$fV$JK2;
  eq$gC$p = eqr$gC$p; eq$fC$p = eqr$fC$p;
  eq$gC$j = eqr$gC$j; eq$fC$j = eqr$fC$j;
  eq$p = eqr$p; evol$eq$p = evol$eqr$p;
  eq$bimConsLaw = eqr$bimConsLaw;
  evol$eq$gA = evol$eqr$gA; evol$eq$gB = evol$eqr$gB;
  evol$eq$gK1 = evol$eqr$gK1; evol$eq$gK2 = evol$eqr$gK2;
  evol$eq$fA = evol$eqr$fA; evol$eq$fB = evol$eqr$fB;
  evol$eq$fK1 = evol$eqr$fK1; evol$eq$fK2 = evol$eqr$fK2;
  eq$gW = eqr$gW; eq$fW = eqr$fW; eq$cW = eqr$cW;
]

defs = "(* Bimetric equations in the case of spherical symmetry *)\n" <>
  "(* Exported:   "<>DateString["ISODateTime"]<> "                                *)\n" <>
  "(* Reference: Geometric mean of bimetric spacetimes      *)\n" <>
  "(*              https://arxiv.org/abs/1803.09752          *)\n\n";

$regularB = False;

defs = defs <> "(* Auxiliary equations *)" <> "\n\n";
appendDefs["eq$Lt", sLt];
appendDefs["eq$v", sLp / sLt];

defs = defs <> "(* Shifted elementary symmetric polynomials *)" <> "\n\n";
defs = defs <> "$Vsign = "<>ToString@$Vsign<> "; \n\n";
defs = defs <> "eq$esP[n_, k_, v_] := "<>
  "Sum[ $Vsign \beta[i+k] * SymmetricPolynomial[ i, Table[v,n] ], {i, 0, n} ]" <> "\n\n";

$regularB = False;
exportDefs[]
defs = defs <> ToString@Definition[useEqn$] <> "\n\n";

```

```
$regularB = True;  
exportDefs[]  
defs = defs <> ToString@Definition[useEqr$] <> "\n\n";  
  
If[$exportDefinitions != False,  
  Export["bimetric-ss-nr.m", defs, "String"];  
]
```

## Part II -- Verification

### Additional definitions

Define a 4D manifold with a chart

```
DefManifold[M4, 4, {a, b, c, d, e}]

scalarsΣt = {t[], r[], θ[], ϕ[]};
scalarsB4 = {xt[], xr[], xθ[], xϕ[]};

DefChart[B4, M4, Range[0, 3], scalarsB4, ChartColor → RGBColor[0.7, 0, 0]]

toB4[expr_] :=
  expr // ToBasis[B4] // ToBasis[B4] // TraceBasisDummy // ComponentArray // ToValues //
  Simplify
```

The metric  $g$

$$g_{\mu\nu} = \frac{-\underline{gAlpha}^2 + \underline{gEA}^2 \underline{gBeta}^2 \left\{ \left\{ \underline{gBeta}, 0, 0 \right\} \cdot \underline{\gamma} \right\}}{\underline{\gamma} \cdot \left\{ \left\{ \underline{gBeta}, 0, 0 \right\} \right\}^T \underline{\gamma}} \quad /.$$

$\{\underline{gBeta} \rightarrow \underline{eq\$gBeta}, \underline{fBeta} \rightarrow \underline{eq\$fBeta}\} // \text{Simplify};$

$g_{\mu\nu} // \text{printNice} // \text{MatrixForm}$

$$\begin{pmatrix} -\alpha^2 + (A q + v \alpha)^2 & A (A q + v \alpha) & 0 & 0 \\ A (A q + v \alpha) & A^2 & 0 & 0 \\ 0 & 0 & B^2 & 0 \\ 0 & 0 & 0 & \sin[\theta]^2 B^2 \end{pmatrix}$$

Setup the metric  $g$  on a manifold  $M_4$  in a basis  $B_4$ ,

```
DefMetric[-1, g[-a, -b], CD, SymbolOfCovD -> {";", "\n"}, PrintAs -> "g"]

CD[a_][β[n_]] := 0

MetricInBasis[g, -B4, g_{\mu\nu} /. Thread[scalarsΣt → scalarsB4]];

MetricCompute[g, B4, "Christoffel"[-1, -1, -1], CVSimplify → Simplify]
MetricCompute[g, B4, "Christoffel"[1, -1, -1], CVSimplify → Simplify]
```

The metric  $f$

$$f_{\mu\nu} = \frac{-\underline{fAlpha}^2 + \underline{fEA}^2 \underline{fBeta}^2 \left\{ \left\{ \underline{fBeta}, 0, 0 \right\} \cdot \underline{\varphi} \right\}}{\underline{\varphi} \cdot \left\{ \left\{ \underline{fBeta}, 0, 0 \right\} \right\}^T \underline{\varphi}} \quad // \text{instantiateBetas} // \text{Simplify};$$

$f_{\mu\nu} // \text{printNice} // \text{MatrixForm}$

$$\begin{pmatrix} -\tilde{\alpha}^2 + (q \tilde{A} - v \tilde{\alpha})^2 & \tilde{A} (q \tilde{A} - v \tilde{\alpha}) & 0 & 0 \\ \tilde{A} (q \tilde{A} - v \tilde{\alpha}) & \tilde{A}^2 & 0 & 0 \\ 0 & 0 & \tilde{B}^2 & 0 \\ 0 & 0 & 0 & \sin[\theta]^2 \tilde{B}^2 \end{pmatrix}$$

Construct the square root

$$\mathbb{E}[\text{vec}_\mu] := \begin{pmatrix} 1 & 0 \\ \text{vec} & \text{SI}_\mu \end{pmatrix}$$

```

□ 
$$\begin{pmatrix} \underline{gAlpha}^{-1} \underline{fAlpha} \underline{sLt}^{-1} & \underline{gAlpha}^{-1} \{ \{ \underline{sLp}, 0, 0 \} \} \cdot \underline{fE} \\ -\underline{fAlpha} \underline{gE}^{-1} \cdot \{ \{ \underline{sLp} / \underline{sLt}^2, 0, 0 \} \}^T & \underline{gE}^{-1} \cdot \underline{sLs}^{-1} \cdot \underline{fE} \end{pmatrix};$$


$$\underline{S} = \mathbb{E} @ \begin{pmatrix} -\underline{hBeta} \\ 0 \\ 0 \end{pmatrix} \cdot \% \cdot \mathbb{E} @ \begin{pmatrix} \underline{hBeta} \\ 0 \\ 0 \end{pmatrix} // \text{instantiateBetas} // \text{convert}\$p2\lambda // \text{FullSimplify};$$


$$\underline{S} // \text{printNice} // \text{MatrixForm}$$


$$\begin{pmatrix} \frac{p q \lambda \tilde{A} + \tilde{a}}{\alpha \lambda} & \frac{p \tilde{A}}{\alpha} & 0 & 0 \\ \frac{g \lambda (\alpha - A p q \lambda) \tilde{A} - (p \alpha + A q \lambda) \tilde{a}}{A \alpha \lambda^2} & \left( -\frac{p q}{\alpha} + \frac{1}{A \lambda} \right) \tilde{A} & 0 & 0 \\ 0 & 0 & \frac{\tilde{B}}{B} & 0 \\ 0 & 0 & 0 & \frac{\tilde{B}}{B} \end{pmatrix}$$


```

Verify the square root,

```


$$\underline{f} = \underline{g} \cdot \underline{S} \cdot \underline{S} / . \underline{sLv} \rightarrow \underline{sLp} / \underline{sLt} / . \underline{sLt} \rightarrow (1 + \underline{sLp}^2)^{1/2} // \text{Expand} // \text{FullSimplify} // \text{printNice} //$$


$$\text{MatrixForm} // \text{Framed}$$


True


```

## The bimetric stress-energy tensor and the potential

```


$$\underline{Vg} = \$Vsign \sum_{n=0}^3 \beta[n] \underline{Y}_n[\underline{S}] // \text{Simplify};$$


$$\underline{Vf} = \$Vsign \sum_{n=0}^3 \beta[4-n] \underline{Y}_n[\underline{\tilde{S}}] // \text{Simplify};$$


$$\underline{Vpot} = \$Vsign \sum_{n=0}^4 \beta[n] \underline{\mathcal{E}}_n[\underline{S}] // \text{Simplify};$$


$$\underline{Vg} + \text{Det}@\underline{S} \underline{Vf} == \underline{Vpot} \text{IdentityMatrix}[4] // \text{Simplify} // \text{Framed}$$


True



DefTensor[Vg[a, -b], M4, PrintAs -> "Vg"]
DefTensor[Vf[a, -b], M4, PrintAs -> "Vf"]

AllComponentValues[Vg[{a, B4}, -{b, B4}], Vg /. Thread[scalarsΣt -> scalarsB4]];
AllComponentValues[Vf[{a, B4}, -{b, B4}], Vf /. Thread[scalarsΣt -> scalarsB4]];

```

## The projections on $\Sigma_t$

The unit normal  $n_g$ , and the projection operator  $\mathbb{P}_g$ ,

```


$$\underline{ng}\$d = \{ \{ -\underline{gAlpha}, 0, 0, 0 \} \};$$


$$\underline{ng}\$u = \left( \{ \{ 1 / \underline{gAlpha}, -\underline{gBeta} / \underline{gAlpha}, 0, 0 \} \}^T // \text{instantiateBetas} \right) / . \underline{sLv} \rightarrow \underline{sLp} / \underline{sLt};$$


$$\underline{Pg}\$ud = \text{IdentityMatrix}[4] + \underline{ng}\$u \cdot \underline{ng}\$d // \text{Simplify};$$

DefTensor[ng[-a], M4, PrintAs -> "ng"]

AllComponentValues[ng[-{a, B4}], Flatten@ng$d /. Thread[scalarsΣt -> scalarsB4]];
AllComponentValues[ng[{a, B4}], Flatten@ng$u /. Thread[scalarsΣt -> scalarsB4]];

DefTensor[Pg[a, -b], M4, PrintAs -> "Pg"]

AllComponentValues[Pg[{a, B4}, -{b, B4}], Pg$dud /. Thread[scalarsΣt -> scalarsB4]];

```

The unit normal  $n_f$ , and the projection operator  $\mathbb{P}_f$ ,

```

nf$d = {{-fAlpha, 0, 0, 0}};
nf$u = ({1/fAlpha, -fBeta/fAlpha, 0, 0})^T // instantiateBetas / . sLv -> sLp / sLt;
Pf$ud = IdentityMatrix[4] + nf$u.nf$d // Simplify;

```

## Verification of $\rho$ [], $j$ [], and $J$ [] for $V_g$ and $V_f$

Here we evaluate the direct projections and compare to the results from the main notebook.

The normal projections of  $V_g$  and  $V_f$ ,

```

rho$Vg = (ng$d.Vg.nf$u)[[1, 1]] // simplifyShiftedESP // convert$p2l;
% // printNice
rho$Vg == gp[] // Simplify // Framed

```

$$-\langle R \rangle_0^2 - \frac{\langle R \rangle_1^2 \lambda \tilde{A}}{A}$$

True

```

rho$Vf = (nf$d.Vf.nf$u)[[1, 1]] // simplifyShiftedESP // convert$p2l;
% // printNice
rho$Vf == fp[] // Simplify // Framed

```

$$-\frac{\langle R \rangle_1^2 A \lambda + \langle R \rangle_2^2 \tilde{A}}{R^2 \tilde{A}}$$

True

The mixed projections of  $V_g$  and  $V_f$  (as a covector),

```

j$Vg = -gamma.V[Pg$ud.Vg.nf$u] // simplifyShiftedESP // convert$p2l // Flatten;
% // printNice
j$Vg == (gj[-i] // toB // Flatten) // Simplify // Framed

```

$$\{-\langle R \rangle_1^2 p \tilde{A}, 0, 0\}$$

True

```

j$Vf = -phi.V[Pf$ud.Vf.nf$u] // simplifyShiftedESP // convert$p2l // Flatten;
% // printNice

```

$$\left\{ \frac{\langle R \rangle_1^2 A p}{R^2}, 0, 0 \right\}$$

The full projections of  $V_g$  and  $V_f$  (as an operator),

```

J$Vg = Pg$ud.Vg.Pg$ud // V // Diagonal // simplifyShiftedESP // convert$p2l // Expand;
% // printNice
J$Vg == (gj[i, -j] // toB // convert$p2l // Diagonal) // Simplify // Framed

```

$$\left\{ \langle R \rangle_0^2 + \frac{\langle R \rangle_1^2 \tilde{A}}{A \lambda} - \frac{\langle R \rangle_1^2 \lambda \tilde{A}}{A} + \frac{\langle R \rangle_1^2 \tilde{\alpha}}{\alpha \lambda}, \langle R \rangle_0^1 + \frac{\langle R \rangle_1^1 \tilde{A}}{A \lambda} + \frac{\langle R \rangle_1^1 \tilde{\alpha}}{\alpha \lambda} + \frac{\langle R \rangle_2^1 \tilde{A} \tilde{\alpha}}{A \alpha}, \langle R \rangle_0^1 + \frac{\langle R \rangle_1^1 \tilde{A}}{A \lambda} + \frac{\langle R \rangle_1^1 \tilde{\alpha}}{\alpha \lambda} + \frac{\langle R \rangle_2^1 \tilde{A} \tilde{\alpha}}{A \alpha} \right\}$$

True

```

gJp == J$Vg - 1/2 (Total@J$Vg - rho$Vg) // Simplify // Framed

```

True

```

J$Vf = Pf$ud.Vf■.Pf$ud // ▼ // Diagonal // simplifyShiftedESP // convert$p2λ // Expand;
% // printNice
J$Vf = (fJ[, -] // toB // convert$p2λ // Diagonal) // Simplify // Framed
{
  <R>_2^2 / R^2 + <R>_1^2 A / R^2 λ ã - <R>_1^2 A λ / R^2 ã + <R>_1^2 α / R^2 λ ã, <R>_3 / R + <R>_2^1 A / R λ ã + <R>_2^1 α / R λ ã + <R>_1^1 A α / R ã ã, <R>_3 / R + <R>_2^1 A / R λ ã + <R>_2^1 α / R λ ã + <R>_1^1 A α / R ã ã
}

True

fJp = J$Vf - 1/2 (Total@J$Vf - ρ$Vf) // Simplify // Framed

True

```

## Verification of eqs (2.35a) and (2.35b)

$$\partial_t \rho - n^i \partial_t j_i = \frac{1}{2} (Q\tilde{u})^{ij} \partial_t \gamma_{ij} - \frac{1}{2} \tilde{u}^{ij} \partial_t \varphi_{ij}, \quad (2.35a)$$

```

ρ$Vg$t = D[ρ$Vg /. sER → fEB / gEB // instantiateShiftedESP, t[]];
j$Vg$t = D[j$Vg /. sER → fEB / gEB // instantiateShiftedESP, t[]];
(ρ$Vg$t - sgn■. {j$Vg$t}^T) [[1, 1]] // convert$p2λ // Simplify;
eq235a$LHS = % /. D[sLt, t[]] → D[sLp, t[]] sLp / sLt // Simplify;

1/2 sgQU■.Inverse@γ■.D[γ■, t[]] - 1/2 sfU■.Inverse@φ■.D[φ■, t[]] // Simplify;
% // convert$p2λ;
Tr[%] // instantiateBetas // Simplify;
Block[{sLv}, sLv[t_, r_] := sLp[t, r] / (1 + sLp[t, r]^2)^{1/2}; %] // Simplify;
eq235a$RHS = % // convert$p2λ;

eq235a$LHS == eq235a$RHS // Simplify // Framed

True

```

$$\partial_k \rho - n^i \partial_k j_i = \frac{1}{2} (Q\tilde{u})^{ij} \partial_k \gamma_{ij} - \frac{1}{2} \tilde{u}^{ij} \partial_k \varphi_{ij}. \quad (2.35b)$$

```

ρ$Vg$r = D[ρ$Vg /. sER → fEB / gEB // instantiateShiftedESP, r[]];
j$Vg$r = D[j$Vg /. sER → fEB / gEB // instantiateShiftedESP, r[]];
(ρ$Vg$r - sgn■. {j$Vg$r}^T) [[1, 1]] // convert$p2λ // Simplify;
eq235b$LHS = % /. D[sLt, r[]] → D[sLp, r[]] sLp / sLt // Simplify;

1/2 sgQU■.Inverse@γ■.D[γ■, r[]] - 1/2 sfU■.Inverse@φ■.D[φ■, r[]] // Simplify;
% // convert$p2λ;
Tr[%] // instantiateBetas // Simplify;
Block[{sLv}, sLv[t_, r_] := sLp[t, r] / (1 + sLp[t, r]^2)^{1/2}; %] // Simplify;
eq235b$RHS = % // convert$p2λ;

eq235b$LHS == eq235b$RHS // Simplify // Framed

True

```

# Verification of the bimetric conservation law

Note that during the projection we only use the EoM for the spatial metrics.

The perpendicular projection  $n_g{}^b \nabla_a V_g{}^a{}_b$ ,

```
ng[b] CD[-a][Vg[a, -b]] // toB4 //
Block[
  {sLv},
  sLv[t_, r_] := sLp[t, r] / sLt[t, r];
  # /. {xt[] -> t[], xr[] -> r[], x0[] -> 0[], xphi[] -> phi[]} //. {
    evol$dot$gSp[[1]] -> evol$eq$gSp[[1]],
    evol$dot$gSp[[2]] -> evol$eq$gSp[[2]],
    evol$dot$fSp[[1]] -> evol$eq$fSp[[1]],
    evol$dot$fSp[[2]] -> evol$eq$fSp[[2]]
  } // instantiateBetas
] & // Simplify;
% /. {D[sLt, t[]] -> D[(1 + sLp^2)^(1/2), t[]], D[sLt, r[]] -> D[(1 + sLp^2)^(1/2), r[]]} // Simplify;
nabla$rho = % /. {1 + sLp^2 -> sLt^2} // Simplify;
```

Solve  $\partial_t p$  from  $\nabla_a \rho$ ,

```
p$t$from$rho = D[sLp, t[]] /. Solve[nabla$rho == 0, D[sLp, t[]]] [[1]] // simplifyShiftedESP;
% // printNice
- 1 /
  <R>_1^2 A B p lambda A-tilde^2
  (p lambda A-tilde (-<R>_1^2 B (partial_r A-tilde alpha lambda + A-tilde (-partial_r alpha lambda + A (partial_r p q + p alpha K_1))) - 2 <R>_1 alpha (-partial_r B lambda A-tilde + A (partial_r B-tilde + B p A-tilde K_2))) -
  A A-tilde (2 partial_r B-tilde <R>_1 A p lambda + B lambda^2 A-tilde^2 (-2 <R>_1^2 K_2 + lambda (-2 <R>_1^2 K-tilde_2 + <R>_1^2 (K-tilde_1 + 2 K-tilde_2))) +
  A-tilde (partial_r p <R>_1^2 B (-p^2 + lambda^2) + lambda (2 partial_r B-tilde <R>_1^2 p lambda + A B (-<R>_1^2 K_1 - 2 <R>_1^2 K_2 + 2 (-<R>_0 + <R>_0) lambda K-tilde_2))))))
```

The mixed projection of  $\mathbb{P}_g{}^b{}_c \nabla_a V_g{}^a{}_b$ ,

```
Pg[b, -c] CD[-a][Vg[a, -b]] // toB4 //
Block[
  {sLv},
  sLv[t_, r_] := sLp[t, r] / sLt[t, r];
  # /. {xt[] -> t[], xr[] -> r[], x0[] -> 0[], xphi[] -> phi[]} //. {
    evol$dot$gSp[[1]] -> evol$eq$gSp[[1]],
    evol$dot$gSp[[2]] -> evol$eq$gSp[[2]],
    evol$dot$fSp[[1]] -> evol$eq$fSp[[1]],
    evol$dot$fSp[[2]] -> evol$eq$fSp[[2]]
  } // instantiateBetas
] & // Simplify;
% /. {D[sLt, t[]] -> D[(1 + sLp^2)^(1/2), t[]], D[sLt, r[]] -> D[(1 + sLp^2)^(1/2), r[]]} // Simplify;
nabla$j = %[[2]] /. {1 + sLp^2 -> sLt^2} // Simplify;
p$t$from$j = D[sLp, t[]] /. Solve[nabla$j == 0, D[sLp, t[]]] [[1]] // simplifyShiftedESP;
% // printNice
1 /
  <R>_1^2 A B A-tilde
  (2 <R>_1^2 (partial_r B-tilde A lambda - partial_r B A-tilde) A-tilde + <R>_1^2 (2 alpha (partial_r B-tilde A + A-tilde (-partial_r B lambda + A B p K_2)) - 2 A B p A-tilde A-tilde K-tilde_2) +
  <R>_1^2 B (partial_r A-tilde alpha lambda + A-tilde (partial_r p A q - partial_r alpha lambda + A p alpha K_1) + A p A-tilde A-tilde (K-tilde_1 + 2 K-tilde_2)))
```

```

(p$t$from$ρ - p$t$from$j // Simplify) /. sLt2 → 1 + sLp2;
Row@{Cbim, " == ", Framed[
$$\frac{-1}{f\alpha} \text{HoldForm}[j_r (\partial_t p_\rho - \partial_t p_j)]$$
, Background → LightYellow]} //
printNice

```

$$CC2Ag + CC2Af + CC2B == \frac{-j\$Vg[[1]]}{f\alpha} \% \quad // \text{ instantiateShiftedESP // Simplify // Framed}$$

$$C_{bim} == - \frac{j_r (\partial_t p_\rho - \partial_t p_j)}{\tilde{\alpha}}$$

True

$$\text{evol\$p} = p\$t\$from\$j \quad // \text{ Simplify // Framed}$$

True

## The two evolution equations for $\partial_t p$

The expressions for  $\partial_t p$ , from  $\rho$ ,

```

p$t$from$ρ3 =
P[2, 1, sER] p$t$from$ρ // Collect[#, {gAlpha, fAlpha, sLp, sLt}, Simplify@Expand@# &] &;
p$t$from$ρ3 // printNice

```

$$\begin{aligned}
& \partial_r p \langle R \rangle_1^2 q + \langle R \rangle_1^2 \lambda \left( -\frac{\partial_r \alpha}{A} + \frac{\partial_r \tilde{\alpha}}{\tilde{A}} \right) + \alpha \left( -\frac{2 \partial_r B \langle R \rangle_1^1 \lambda}{A B} + \frac{2 \partial_r \tilde{B} \langle R \rangle_1^1}{B \tilde{A}} + p \left( \langle R \rangle_1^2 K_1 + 2 \langle R \rangle_1^1 K_2 \right) \right) + \\
& \tilde{\alpha} \left( \frac{2 \partial_r \tilde{B} \langle R \rangle_1^1 A}{B \tilde{A}^2} - \frac{\partial_r p \langle R \rangle_1^2 p}{\lambda \tilde{A}} + \frac{2 \partial_r \tilde{B} \langle R \rangle_2^1 \lambda}{B \tilde{A}} + \frac{1}{p} \left( -\frac{A \left( \langle R \rangle_1^2 K_1 + 2 \langle R \rangle_1^1 K_2 \right)}{\tilde{A}} + \right. \right. \\
& \quad \left. \left. \lambda^2 \left( \langle R \rangle_1^2 \tilde{K}_1 - 2 \left( \langle R \rangle_1^1 - \langle R \rangle_1^2 \right) \tilde{K}_2 \right) + \frac{1}{\tilde{A}} \lambda \left( \partial_r p \langle R \rangle_1^2 - 2 \langle R \rangle_2^1 \tilde{A} K_2 + 2 \left( -\langle R \rangle_0^1 + \langle R \rangle_0^2 \right) A \tilde{K}_2 \right) \right) \right)
\end{aligned}$$

The expressions for  $\partial_t p$ , from  $j$ ,

```

p$t$from$j3 = P[2, 1, sER] p$t$from$j // Collect[#, {gAlpha, fAlpha, sLp, sLt}, Simplify] &;
p$t$from$j3 // printNice

```

$$\begin{aligned}
& \partial_r p \langle R \rangle_1^2 q + \langle R \rangle_1^2 \lambda \left( -\frac{\partial_r \alpha}{A} + \frac{\partial_r \tilde{\alpha}}{\tilde{A}} \right) + \alpha \left( -\frac{2 \partial_r B \langle R \rangle_1^1 \lambda}{A B} + \frac{2 \partial_r \tilde{B} \langle R \rangle_1^1}{B \tilde{A}} + p \left( \langle R \rangle_1^2 K_1 + 2 \langle R \rangle_1^1 K_2 \right) \right) + \\
& \tilde{\alpha} \left( -\frac{2 \partial_r B \langle R \rangle_2^1}{A B} + \frac{2 \partial_r \tilde{B} \langle R \rangle_2^1 \lambda}{B \tilde{A}} + p \left( \langle R \rangle_1^2 \tilde{K}_1 - 2 \left( \langle R \rangle_1^1 - \langle R \rangle_1^2 \right) \tilde{K}_2 \right) \right)
\end{aligned}$$



## Verification of the symmetric form of $C_{\text{bim}}$ in (D.17)

$$\text{term1} = \text{sgU}[i, -j] \left( \text{cdg}[-i][\text{sgn}[j]] - \frac{1}{2} \text{ChristoffelcdgPD}\Sigma\text{B}[k, -k, -i] \text{sgn}[j] - \text{gK}[j, -i] \right)$$

$$\text{term2} = \text{sfU}[i, -j] \left( \text{cdf}[-i][\text{sfn}[j]] + \frac{1}{2} \text{ChristoffelcdfPD}\Sigma\text{B}[k, -k, -i] \text{sfn}[j] + \text{fK}[j, -i] \right)$$

$$\text{term3} = \left( \frac{1}{2} \text{cdg}[-i][\text{sgU}[i, -j] \text{sgn}[j]] + \frac{1}{2} \text{cdf}[-i][\text{sfU}[i, -j] \text{sfn}[j]] \right)$$

$$\mathcal{U}^i{}_j \left( -K^j{}_i - \frac{1}{2} \Gamma[\mathcal{D}, \mathcal{D}]^k{}_{ki} n^j + \mathcal{D}_i n^j \right)$$

$$\tilde{\mathcal{U}}^i{}_j \left( \tilde{K}^j{}_i + \frac{1}{2} \Gamma[\tilde{\mathcal{D}}, \mathcal{D}]^k{}_{ki} \tilde{n}^j + \tilde{\mathcal{D}}_i \tilde{n}^j \right)$$

$$\frac{1}{2} \left( \tilde{\mathcal{U}}^i{}_j (\tilde{\mathcal{D}}_i \tilde{n}^j) + \tilde{n}^j (\tilde{\mathcal{D}}_i \tilde{\mathcal{U}}^i{}_j) \right) + \frac{1}{2} \left( \mathcal{U}^i{}_j (\mathcal{D}_i n^j) + n^j (\mathcal{D}_i \mathcal{U}^i{}_j) \right)$$

$$\text{term4} = \text{sgU}[i, -j] \text{cdg}[-i][\text{sgn}[j]] - \text{sgU}[i, -j] \text{gK}[j, -i]$$

$$\text{term5} = \text{sfU}[i, -j] \text{cdf}[-i][\text{sfn}[j]] + \text{sfU}[i, -j] \text{fK}[j, -i]$$

$$\text{term6} = \text{cdg}[-i][\text{sgU}[i, -j] \text{sgn}[j]]$$

$$-K^j{}_i \mathcal{U}^i{}_j + \mathcal{U}^i{}_j (\mathcal{D}_i n^j)$$

$$\tilde{K}^j{}_i \tilde{\mathcal{U}}^i{}_j + \tilde{\mathcal{U}}^i{}_j (\tilde{\mathcal{D}}_i \tilde{n}^j)$$

$$\mathcal{U}^i{}_j (\mathcal{D}_i n^j) + n^j (\mathcal{D}_i \mathcal{U}^i{}_j)$$

$$\left( \left( \text{term1} + \text{term2} - \text{term3} \right) - \left( \text{term4} + \text{term5} - \text{term6} \right) \right) // \text{toB} // \text{convert}\$K) /. \{1 + \text{sLp}^2 \rightarrow \text{sLt}^2\} //$$

Simplify // Expand;

% ==

0 //

Framed

True

$$(\text{sLt gEA}(\text{term1} + \text{term2} - \text{term3}) // \text{toB} // \text{convert}\$K) /. \{1 + \text{sLp}^2 \rightarrow \text{sLt}^2\} // \text{Simplify} // \text{Expand};$$

$$\text{CC2Ag} + \text{CC2Af} + \text{CC2B} /. \text{sER} \rightarrow \text{fEB} / \text{gEB} // \text{toB} // \text{instantiateShiftedESP} // \text{Expand};$$

%% - % == 0 // Framed

True
