# Supplementary material for: On the ratio of lapses in bimetric relativity
Source: arXiv:1903.09646 ancillary file (2019-03-22)
Supplement: Supplementary file 3 [file 02-lapse-ratio.pdf]

# Bimetric equations in standard 3+1 form reduced to spherical symmetry (lapse ratio)

Mikica Kocic, created 2018-05-14, last modified 2019-02-19

Calculation of the lapse ratio by expanding the preservation of the bimetric conservation law. Evaluation of this notebook creates the package "bimetric-ss-nr.m".

## Requirements:

Evaluation of this notebook requires the package "bimetric-lapses-nr.m".

## Changelog:

2018-05-14 The initial release.

2018-09-08 Emitted the overall factor into the module.

2019-02-19 Generated eqn\$gW2, eqn\$fW2 that contain only the first derivatives of  $B$  and  $\tilde{B}$

---

## Definitions

### The prerequisite packages

```
SetDirectory@NotebookDirectory[];
<< "bimetric-ss-nr.m"

Style[Row@{"The V-sign convention is: ", If[$Vsign > 0, "+", ""], $Vsign}, Bold, Red]
The V-sign convention is: -1

useEqn$[]
```

### Additional definitions

```
 $f_{\underline{t}}$  := f[t, r]

esP$rule := P[n_, k_, ev_] => eq$esP[n, k, ev]

Lt$r$rule = D[Lt, r] -> (D[(1 + p^2)^(1/2), r] /. p^2 -> Lt^2 - 1 // Simplify[#, Assumptions -> Lt >= 1] &);

instantiateBetas[e_] := Block[{gBet, fBet},
  gBet[t_, r_] := eq$gBet[t, r];
  fBet[t_, r_] := eq$fBet[t, r];
  e
]

$Assumptions = True;
```

```

printNice[e_, esP_ : P] := e /. {
  gA → Style[A, Blue], gB → Style[B, Blue], gK1 → Style[K1, Blue], gK2 → Style[K2, Blue],
  fA → Style[ $\tilde{A}$ , Red], fB → Style[ $\tilde{B}$ , Red], fK1 → Style[ $\tilde{K}_1$ , Red], fK2 → Style[ $\tilde{K}_2$ , Red],
  gAlp → Style[ $\alpha$ , Blue], gBet → Style[ $\beta$ , Blue], fAlp → Style[ $\tilde{\alpha}$ , Red], fBet → Style[ $\tilde{\beta}$ , Red],
  R → Style[R, Magenta], q → Style[q, Darker@Green], rhoPF → Style[oPF, Purple],
  p → Style[p, Darker@Green], v → Style[v, Darker@Green], Lt → Style[ $\lambda$ , Darker@Green],
  g$ρ → Framed[gρ, Background → LightBlue],
  g$JK1 → Framed[gJK1, Background → LightBlue],
  g$JK2 → Framed[gJK2, Background → LightBlue],
  f$ρ → Framed[fρ, Background → LightRed],
  f$JK1 → Framed[fJK1, Background → LightRed],
  f$JK2 → Framed[fJK2, Background → LightRed],
  gT$ρ → Style[Tρ, Darker@Red], gT$j → Style[Tj, Darker@Red],
  gT$JK1 → Style[TJ1, Darker@Red], gT$JK2 → Style[TJ2, Darker@Red],
  fT$ρ → Style[ $\tilde{T}\rho$ , Darker@Red], fT$j → Style[ $\tilde{T}j$ , Darker@Red],
  fT$JK1 → Style[ $\tilde{T}J_1$ , Darker@Blue], fT$JK2 → Style[ $\tilde{T}J_2$ , Darker@Blue],
  k$g → Style[kg, Blue], k$f → Style[kf, Red], β[n_] := βn,
  F[n_] := Fn, G[n_] := Gn
} //. {
Derivative[0, 1][f_][t, r] := HoldForm[ $\partial_r f$ ],
Derivative[0, 2][f_][t, r] := HoldForm[ $\partial_{rr} f$ ],
Derivative[1, 0][f_][t, r] := HoldForm[ $\partial_t f$ ],
Derivative[2, 0][f_][t, r] := HoldForm[ $\partial_{tt} f$ ],
Derivative[1, 1][f_][t, r] := HoldForm[ $\partial_{tr} f$ ],
f_[t, r] := f,
esP[n_, k_, R_] := HoldForm[ $\langle R \rangle_k^n$ ]
}

```

# The relation between two lapses

The bimetric conservation law (it is established by projecting nabla of the bimetric potential),

```
eq$bimConsLaw // printNice // Framed
```

$$\frac{\partial_r p \langle R \rangle_1^2}{\lambda} + \frac{2 \partial_r \tilde{B} \langle R \rangle_1^1 A p}{B \tilde{A}} + \tilde{A} \left( 2 \langle R \rangle_2^1 \left( \frac{\partial_r B p}{A B} - \lambda K_2 \right) + \langle R \rangle_1^2 \tilde{K}_1 + 2 \left( -\langle R \rangle_1^1 + \langle R \rangle_1^2 \right) \tilde{K}_2 \right) - A \left( \langle R \rangle_1^2 K_1 + 2 \langle R \rangle_1^1 \left( K_2 - R \lambda \tilde{K}_2 \right) \right)$$

The evolution equation for  $p$ ,

```
evol$eq$p P[2, 1, R] // Collect[#, {gAlp, fAlp, p, Lt}, Simplify] & // printNice // Framed
```

$$\partial_r p \langle R \rangle_1^2 q + \langle R \rangle_1^2 \lambda \left( -\frac{\partial_r \alpha}{A} + \frac{\partial_r \tilde{\alpha}}{\tilde{A}} \right) + \alpha \left( -\frac{2 \partial_r B \langle R \rangle_1^1 \lambda}{A B} + \frac{2 \partial_r \tilde{B} \langle R \rangle_1^1}{B \tilde{A}} + p \left( \langle R \rangle_1^2 K_1 + 2 \langle R \rangle_1^1 K_2 \right) \right) + \tilde{\alpha} \left( -\frac{2 \partial_r B \langle R \rangle_2^1}{A B} + \frac{2 \partial_r \tilde{B} \langle R \rangle_2^1 \lambda}{B \tilde{A}} + p \left( \langle R \rangle_1^2 \tilde{K}_1 - 2 \left( \langle R \rangle_1^1 - \langle R \rangle_1^2 \right) \tilde{K}_2 \right) \right)$$

## Build a time derivative of the bimetric conservation law

```
step$1 = D[eq$bimConsLaw[t, r] // Expand, t] /. {
  Derivative[1, 0][R][t, r] => Framed[D[fB / gB, t], Background -> LightBlue],
  Derivative[1, 0][Lt][t, r] => Framed[p D[p, t] / Lt, Background -> LightCyan],
  Derivative[1, 0][p][t, r] => Framed[evol$eq$p, Background -> LightGreen],
  Derivative[1, 1][p][t, r] => Framed[D[evol$eq$p, r], Background -> GrayLevel[0.98]],
  Derivative[0, 0, 1][P][0, k_, R_] => Framed[0, Background -> LightMagenta],
  Derivative[0, 0, 1][P][1, k_, R_] => Framed[P[0, k + 1, R], Background -> LightMagenta],
  Derivative[0, 0, 1][P][2, k_, R_] => Framed[2 P[1, k + 1, R], Background -> LightMagenta]
} /. {
  Derivative[1, 0][p][t, r] => Framed[Derivative[1, 0][p][t, r], Background -> LightRed],
  Derivative[1, 0][f_][t, r] =>
    Framed[Derivative[1, 0][f][t, r], Background -> LightYellow]
};
% // printNice;

step$2 = step$1 /. {Framed[e_, o___] => e} // Expand // Simplify;
```

## Expand and recollect all the terms factored by derivatives

```
Clear[nF, F, Fvalue];
nF = 0;
step$3 = Collect[
  Numerator@step$2,
  Derivative[1, n_][f_][t_, r_],
  {nF = nF + 1; Fvalue[nF] = Simplify@#; F[nF]} &
];
```

```
step$3 /. Derivative[1, n_][f_][t_, r_] := Derivative[1, n][
  Framed[f, Background -> If[n > 0, Yellow, White]]][t, r] // printNice // Framed
```

$$\partial_t \tilde{A} F_1 + \partial_t \tilde{B} F_2 + \partial_t \tilde{K}_1 F_3 + \partial_t \tilde{K}_2 F_4 + \partial_t A F_5 + \\ \partial_t B F_6 + \partial_t K_1 F_7 + \partial_t K_2 F_8 + \partial_{tr} \tilde{B} F_9 + \partial_{tr} B F_{10} + F_{11}$$

```
Do[Echo@Row@printNice@
  {F[n], " == ", Collect[Fvalue[n], {D[q, r], q}, Simplify] /. q -> Framed@q}, {n, nF}]
```

$$\begin{aligned}
\gg F_1 &= \langle R \rangle_1^2 A B^2 \lambda^3 \left( -2 \partial_r \tilde{B} \langle R \rangle_1^2 A^2 p + \tilde{A}^2 \left( 2 \partial_r B \langle R \rangle_1^2 p + A B \left( -2 \langle R \rangle_1^2 \lambda K_2 + \langle R \rangle_1^2 \tilde{K}_1 \right) + 2 \left( -\langle R \rangle_1^2 + \langle R \rangle_1^2 \right) A B \tilde{K}_2 \right) \right) \\
\gg F_2 &= 2 \langle R \rangle_1^2 A B \lambda^2 \tilde{A} \left( \partial_r \tilde{B} \langle R \rangle_2^0 A^2 p \lambda + \lambda \tilde{A}^2 \left( \partial_r B \langle R \rangle_3^0 p + A B \left( -\langle R \rangle_3^0 \lambda K_2 + \langle R \rangle_2^1 \tilde{K}_1 \right) - \left( \langle R \rangle_2^0 - 2 \langle R \rangle_2^1 \right) A B \tilde{K}_2 \right) + \right. \\
&\quad \left. A B \tilde{A} \left( \partial_r p \langle R \rangle_2^1 + A \lambda \left( -\langle R \rangle_2^1 K_1 - \langle R \rangle_2^0 K_2 + \left( \langle R \rangle_1^1 + \langle R \rangle_2^0 \right) R \right) \lambda \tilde{K}_2 \right) \right) \\
\gg F_3 &= \left( \langle R \rangle_1^2 \right)^2 A^2 B^3 \lambda^3 \tilde{A}^3 \\
\gg F_4 &= 2 \langle R \rangle_1^2 A^2 B^3 \lambda^3 \tilde{A}^2 \left( \langle R \rangle_1^1 A R \lambda + \left( -\langle R \rangle_1^1 + \langle R \rangle_1^2 \right) \tilde{A} \right) \\
\gg F_5 &= -\langle R \rangle_1^2 B^2 \lambda^3 \tilde{A} \left( -2 \partial_r \tilde{B} \langle R \rangle_1^2 A^2 p + 2 \partial_r B \langle R \rangle_2^1 p \tilde{A}^2 + A^2 B \tilde{A} \left( \langle R \rangle_1^2 K_1 + 2 \langle R \rangle_1^1 K_2 - 2 \langle R \rangle_1^1 R \lambda \tilde{K}_2 \right) \right) \\
\gg F_6 &= 2 \langle R \rangle_1^2 A \lambda^2 \tilde{A} \left( -\partial_r \tilde{B} A^2 p \lambda \left( \langle R \rangle_1^1 B + \langle R \rangle_2^0 \tilde{B} \right) + \right. \\
&\quad \left. \lambda \tilde{A}^2 \left( -\partial_r B \langle R \rangle_2^1 B p + \tilde{B} \left( -\partial_r B \langle R \rangle_3^0 p + A B \left( \langle R \rangle_3^0 \lambda K_2 - \langle R \rangle_2^1 \tilde{K}_1 \right) + \left( \langle R \rangle_2^0 - 2 \langle R \rangle_2^1 \right) A B \tilde{K}_2 \right) \right) + \right. \\
&\quad \left. A B \tilde{A} \tilde{B} \left( -\partial_r p \langle R \rangle_2^1 + A \lambda \left( \langle R \rangle_2^1 K_1 + \langle R \rangle_2^0 K_2 - \left( \langle R \rangle_1^1 + \langle R \rangle_2^0 \right) R \right) \lambda \tilde{K}_2 \right) \right) \\
\gg F_7 &= -\left( \langle R \rangle_1^2 \right)^2 A^3 B^3 \lambda^3 \tilde{A}^2 \\
\gg F_8 &= -2 \langle R \rangle_1^2 A^2 B^3 \lambda^3 \tilde{A}^2 \left( \langle R \rangle_1^1 A + \langle R \rangle_2^1 \lambda \tilde{A} \right) \\
\gg F_9 &= 2 \langle R \rangle_1^1 \langle R \rangle_1^2 A^3 B^2 p \lambda^3 \tilde{A} \\
\gg F_{10} &= 2 \langle R \rangle_1^2 \langle R \rangle_2^1 A B^2 p \lambda^3 \tilde{A}^3 \\
\gg F_{11} &= \partial_r \boxed{q} \partial_r p \left( \langle R \rangle_1^2 \right)^2 A^2 B^3 \lambda^2 \tilde{A}^2 + \boxed{q} \langle R \rangle_1^2 A B^2 \tilde{A} \left( 2 \partial_r p \partial_r \tilde{B} \langle R \rangle_1^2 A^2 \lambda^3 + \right. \\
&\quad 2 \partial_r p \langle R \rangle_2^1 \lambda^2 \tilde{A}^2 \left( \partial_r B \lambda - A B p K_2 \right) + A B \tilde{A} \left( \langle R \rangle_1^2 \left( -\left( \partial_r p \right)^2 p + \partial_{rr} p \lambda^2 \right) + 2 \partial_r p \langle R \rangle_1^1 A p R \lambda^2 \tilde{K}_2 \right) \Big) + \\
&\quad B \left( -A^2 \lambda^2 \left( \partial_r \tilde{A} \langle R \rangle_1^2 B - 2 \partial_r \tilde{B} \langle R \rangle_1^1 A \lambda \right) \left( \partial_r \tilde{\alpha} \langle R \rangle_1^2 B \lambda + 2 \partial_r \tilde{B} \left( \langle R \rangle_1^1 \alpha + \langle R \rangle_2^1 \lambda \tilde{\alpha} \right) \right) + \right. \\
&\quad A^2 \tilde{A} \left( -2 \partial_r p \partial_r \tilde{B} \langle R \rangle_1^1 \langle R \rangle_1^2 B p \alpha - \partial_r p \partial_r \tilde{\alpha} \left( \langle R \rangle_1^2 \right)^2 B^2 p \lambda + 2 \partial_r \alpha \partial_r \tilde{B} \langle R \rangle_1^1 \langle R \rangle_1^2 B \lambda^2 + \right. \\
&\quad \partial_r \lambda \partial_r \tilde{\alpha} \left( \langle R \rangle_1^2 \right)^2 B^2 \lambda^2 - 2 \partial_r B \partial_r \tilde{B} \langle R \rangle_1^1 \langle R \rangle_1^2 \alpha \lambda^2 + 2 \partial_{rr} \tilde{B} \langle R \rangle_1^1 \langle R \rangle_1^2 B \alpha \lambda^2 + 2 \partial_r R \partial_r \tilde{B} \langle R \rangle_1^1 \langle R \rangle_2^0 B \alpha \lambda^2 - \\
&\quad 4 \partial_r R \partial_r \tilde{B} \langle R \rangle_1^1 \langle R \rangle_2^1 B \alpha \lambda^2 + 2 \partial_r \tilde{B} \partial_r \tilde{\alpha} \langle R \rangle_1^2 \langle R \rangle_2^1 B \lambda^3 + \partial_{rr} \tilde{\alpha} \left( \langle R \rangle_1^2 \right)^2 B^2 \lambda^3 - 2 \partial_r \alpha \partial_r \tilde{B} \langle R \rangle_1^1 \langle R \rangle_1^2 B \lambda^4 - \\
&\quad 4 \partial_r B \partial_r \tilde{B} \left( \langle R \rangle_1^1 \right)^2 \alpha \lambda^4 - 2 \partial_r p \partial_r \tilde{B} \langle R \rangle_1^2 \langle R \rangle_2^1 B p \lambda \tilde{\alpha} + 2 \partial_r \lambda \partial_r \tilde{B} \langle R \rangle_1^2 \langle R \rangle_2^1 B \lambda^2 \tilde{\alpha} - \\
&\quad 4 \partial_r B \partial_r \tilde{B} \langle R \rangle_1^1 \langle R \rangle_2^1 \lambda^3 \tilde{\alpha} - 2 \partial_r B \partial_r \tilde{B} \langle R \rangle_1^2 \langle R \rangle_2^1 \lambda^3 \tilde{\alpha} + 2 \partial_{rr} \tilde{B} \langle R \rangle_1^2 \langle R \rangle_2^1 B \lambda^3 \tilde{\alpha} - 4 \partial_r R \partial_r \tilde{B} \left( \langle R \rangle_2^1 \right)^2 B \lambda^3 \tilde{\alpha} + \\
&\quad 2 \partial_r R \partial_r \tilde{B} \langle R \rangle_1^2 \langle R \rangle_3^0 B \lambda^3 \tilde{\alpha} + 2 \partial_r \tilde{B} \langle R \rangle_1^1 A B p \lambda^3 \left( \alpha \left( \langle R \rangle_1^2 K_1 + 2 \langle R \rangle_1^1 K_2 \right) + \langle R \rangle_1^2 \tilde{\alpha} \tilde{K}_1 \right) + \\
&\quad 2 \langle R \rangle_1^1 A B p \lambda^2 \left( \partial_r \tilde{\alpha} \langle R \rangle_1^2 B R \lambda + 2 \partial_r \tilde{B} \left( \langle R \rangle_1^1 R \alpha + \left( -\langle R \rangle_1^1 + \langle R \rangle_1^2 + \langle R \rangle_2^1 \right) R \right) \lambda \tilde{\alpha} \right) \tilde{K}_2 \Big) + \\
&\quad 2 \langle R \rangle_2^1 \lambda^2 \tilde{A}^3 \left( -\partial_r B \lambda + A B p K_2 \right) \left( \left( \partial_r \alpha \langle R \rangle_1^2 B + 2 \partial_r B \langle R \rangle_1^1 \alpha \right) \lambda - A B p \alpha \left( \langle R \rangle_1^2 K_1 + 2 \langle R \rangle_1^1 K_2 \right) + \right. \\
&\quad \tilde{\alpha} \left( 2 \partial_r B \langle R \rangle_2^1 - \langle R \rangle_1^2 A B p \tilde{K}_1 + 2 \left( \langle R \rangle_1^1 - \langle R \rangle_1^2 \right) A B p \tilde{K}_2 \right) \Big) + \\
&\quad \tilde{A}^2 \left( \partial_r p \partial_r \alpha \left( \langle R \rangle_1^2 \right)^2 A B^2 p \lambda + 2 \partial_r B \partial_r p \langle R \rangle_1^1 \langle R \rangle_1^2 A B p \alpha \lambda - 2 \partial_r B \partial_r \tilde{\alpha} \langle R \rangle_1^2 \langle R \rangle_2^1 A B \lambda^2 - \right. \\
&\quad \partial_r \alpha \partial_r \lambda \left( \langle R \rangle_1^2 \right)^2 A B^2 \lambda^2 - 2 \partial_r B \partial_r \lambda \langle R \rangle_1^1 \langle R \rangle_1^2 A B \alpha \lambda^2 + 2 \partial_r K_2 \langle R \rangle_1^1 \langle R \rangle_1^2 A^2 B^2 p \alpha \lambda^2 + \\
&\quad \partial_r K_1 \left( \langle R \rangle_1^2 \right)^2 A^2 B^2 p \alpha \lambda^2 - 2 \partial_r B \partial_r \alpha \langle R \rangle_1^1 \langle R \rangle_1^2 A B \lambda^3 + \partial_r A \partial_r \alpha \left( \langle R \rangle_1^2 \right)^2 B^2 \lambda^3 - \partial_{rr} \alpha \left( \langle R \rangle_1^2 \right)^2 A B^2 \lambda^3 + \\
&\quad 2 \left( \partial_r B \right)^2 \langle R \rangle_1^1 \langle R \rangle_1^2 A \alpha \lambda^3 + 4 \partial_r B \partial_r \tilde{B} \langle R \rangle_1^1 \langle R \rangle_2^1 A \alpha \lambda^3 + 2 \partial_r A \partial_r B \langle R \rangle_1^1 \langle R \rangle_1^2 B \alpha \lambda^3 - \\
&\quad 2 \partial_{rr} B \langle R \rangle_1^1 \langle R \rangle_1^2 A B \alpha \lambda^3 - 2 \partial_r B \partial_r R \langle R \rangle_1^2 \langle R \rangle_2^0 A B \alpha \lambda^3 + 4 \partial_r B \partial_r R \langle R \rangle_1^1 \langle R \rangle_2^1 A B \alpha \lambda^3 + \\
&\quad 2 \partial_r B \partial_r \tilde{\alpha} \langle R \rangle_1^2 \langle R \rangle_2^1 A B \lambda^4 - \partial_r p \left( \langle R \rangle_1^2 \right)^2 A^2 B^2 p^2 \alpha K_1 + \partial_r \alpha \left( \langle R \rangle_1^2 \right)^2 A^2 B^2 p \lambda^2 K_1 + \\
&\quad \partial_r p \left( \langle R \rangle_1^2 \right)^2 A^2 B^2 \alpha \lambda^2 K_1 - 2 \partial_r p \langle R \rangle_1^1 \langle R \rangle_1^2 A^2 B^2 p^2 \alpha K_2 + 2 \partial_r \alpha \langle R \rangle_1^1 \langle R \rangle_1^2 A^2 B^2 p \lambda^2 K_2 + \\
&\quad 2 \partial_r p \langle R \rangle_1^1 \langle R \rangle_1^2 A^2 B^2 \alpha \lambda^2 K_2 - 4 \partial_r \tilde{B} \langle R \rangle_1^1 \langle R \rangle_2^1 A^2 B p \alpha \lambda^2 K_2 + 2 \partial_r R \langle R \rangle_1^2 \langle R \rangle_2^0 A^2 B^2 p \alpha \lambda^2 K_2 - \\
&\quad 4 \partial_r R \langle R \rangle_1^1 \langle R \rangle_2^1 A^2 B^2 p \alpha \lambda^2 K_2 - 2 \partial_r \tilde{\alpha} \langle R \rangle_1^2 \langle R \rangle_2^1 A^2 B^2 p \lambda^3 K_2 + \partial_r \tilde{\alpha} \left( \langle R \rangle_1^2 \right)^2 A^2 B^2 p \lambda^2 \tilde{K}_1 - \\
&\quad 2 \partial_r \tilde{\alpha} \langle R \rangle_1^1 \langle R \rangle_1^2 A^2 B^2 p \lambda^2 \tilde{K}_2 + 2 \partial_r \tilde{\alpha} \left( \langle R \rangle_1^2 \right)^2 A^2 B^2 p \lambda^2 \tilde{K}_2 - 2 \partial_r \alpha \langle R \rangle_1^1 \langle R \rangle_1^2 A^2 B^2 p R \lambda^3 \tilde{K}_2 - \\
&\quad 4 \partial_r B \left( \langle R \rangle_1^1 \right)^2 A^2 B p R \alpha \lambda^3 \tilde{K}_2 + 2 \langle R \rangle_1^1 \langle R \rangle_1^2 A^3 B^2 p^2 R \alpha \lambda^2 K_1 \tilde{K}_2 + 4 \left( \langle R \rangle_1^1 \right)^2 A^3 B^2 p^2 R \alpha \lambda^2 K_2 \tilde{K}_2 + \\
&\quad \tilde{\alpha} \left( 2 \partial_r A \partial_r B \langle R \rangle_1^2 \langle R \rangle_2^1 B \lambda^2 + 2 A \left( \partial_r B \partial_r p \langle R \rangle_1^2 \langle R \rangle_2^1 B p + \left( 2 \partial_r B \partial_r R \left( \langle R \rangle_2^1 \right)^2 B - \partial_r B \partial_r R \langle R \rangle_1^2 \langle R \rangle_3^0 B + \right. \right. \right. \\
&\quad \left. \left. \left. \langle R \rangle_1^2 \langle R \rangle_2^1 \left( \left( \partial_r B \right)^2 - \partial_{rr} B B \right) \right) \lambda^2 + 2 \partial_r B \partial_r \tilde{B} \left( \langle R \rangle_2^1 \right)^2 \lambda^4 \right) + A^2 B \left( -4 \partial_r \tilde{B} \left( \langle R \rangle_2^1 \right)^2 p \lambda^3 K_2 + \right. \right. \\
&\quad \left. \left. \langle R \rangle_1^2 B \left( -\partial_r p \langle R \rangle_1^2 p^2 \tilde{K}_1 + \lambda^2 \left( \left( -2 \partial_r \tilde{K}_2 \langle R \rangle_1^1 + \left( \partial_r \tilde{K}_1 + 2 \partial_r \tilde{K}_2 \right) \langle R \rangle_1^2 \right) p + \partial_r p \langle R \rangle_1^2 \tilde{K}_1 \right) \right) \right) + 2 A^2 B \right. \\
&\quad \left. \left( \partial_r p \left( \langle R \rangle_1^1 - \langle R \rangle_1^2 \right) \langle R \rangle_1^2 B p^2 - \left( \partial_r p \left( \langle R \rangle_1^1 - \langle R \rangle_1^2 \right) \langle R \rangle_1^2 B + p \left( \partial_r R \langle R \rangle_1^2 \langle R \rangle_2^0 B + 2 \langle R \rangle_1^1 \langle R \rangle_2^1 \left( -\partial_r R B + \right. \right. \right. \right. \right. \\
&\quad \left. \left. \left. \partial_r B R \right) \right) \right) \lambda^2 + \langle R \rangle_1^1 \langle R \rangle_1^2 A B p^2 R \lambda^2 \tilde{K}_1 \right) \tilde{K}_2 + 4 \langle R \rangle_1^1 \left( -\langle R \rangle_1^1 + \langle R \rangle_1^2 \right) A^3 B^2 p^2 R \lambda^2 \tilde{K}_2^2 \Big) \Big)
\end{aligned}$$

During derivation, we will also accumulate the overall factor for each step (factor\$1, factor\$2, ...):

```
corr$factor = Denominator@step$2; (* correction factor applied to the step *)
```

```
factor$2 = corr$factor;
```

```
factor$2 // printNice
```

$$\langle R \rangle_1^2 A^2 B^3 \lambda^3 \tilde{A}^2$$

## Replace the derivatives with the equations of motion

```

step$4 = step$3 /. {
  Derivative[1, k_][gA][t, r] => D[evol$eq$gA, {r, k}],
  Derivative[1, k_][gB][t, r] => D[evol$eq$gB, {r, k}],
  Derivative[1, k_][gK1][t, r] => D[evol$eq$gK1, {r, k}],
  Derivative[1, k_][gK2][t, r] => D[evol$eq$gK2, {r, k}],
  Derivative[1, k_][fA][t, r] => D[evol$eq$fA, {r, k}],
  Derivative[1, k_][fB][t, r] => D[evol$eq$fB, {r, k}],
  Derivative[1, k_][fK1][t, r] => D[evol$eq$fK1, {r, k}],
  Derivative[1, k_][fK2][t, r] => D[evol$eq$fK2, {r, k}],
  Derivative[1, k_][R][t, r] => D[fB / gB, {t, 1}, {r, k}]
} // instantiateBetas // Expand // Collect[#, {
  gAlp[t_, r_], fAlp[t_, r_],
  Derivative[0, n_][gAlp][t_, r_], Derivative[0, n_][fAlp][t_, r_]
},
  Framed@Simplify@# &] &;

% // printNice

```

$$\partial_r q \tilde{A} F_1 + \partial_r q A F_5 + \partial_r q \partial_r \tilde{B} F_9 + \partial_r B \partial_r q F_{10} + q \left( \partial_r \tilde{A} F_1 + \partial_r \tilde{B} F_2 + \partial_r \tilde{K}_1 F_3 + \partial_r \tilde{K}_2 F_4 + \partial_r A F_5 + \partial_r B F_6 + \partial_r K_1 F_7 + \partial_r K_2 F_8 + \partial_{rr} \tilde{B} F_9 + \partial_{rr} B F_{10} \right) + F_{11} +$$

$$\frac{\partial_r A F_7}{A^3} - \frac{\partial_r B F_8}{A^2 B} - B K_2 F_{10} + v \left( F_5 + \frac{\partial_r B F_{10}}{A} \right) \partial_r \alpha + \left( -\frac{F_7}{A^2} \right) \partial_{rr} \alpha +$$

$$\frac{\partial_r \tilde{A} F_3}{\tilde{A}^3} - \frac{\partial_r \tilde{B} F_4}{\tilde{A}^2 \tilde{B}} - \tilde{B} \tilde{K}_2 F_9 + v \left( -F_1 - \frac{\partial_r \tilde{B} F_9}{\tilde{A}} \right) \partial_r \tilde{\alpha} + \left( -\frac{F_3}{\tilde{A}^2} \right) \partial_{rr} \tilde{\alpha} +$$

$$\frac{1}{A^3 B^2} \left( -A^4 B^2 K_1 F_5 + \partial_r A \partial_r B B (2 F_7 + F_8) - A \left( (\partial_r B)^2 F_8 + \partial_{rr} B B (2 F_7 + F_8) + \partial_r A \partial_r B B^2 v F_{10} \right) + A^2 B^2 (\partial_r B \partial_r v F_{10} + v (\partial_r B F_6 + \partial_r K_1 F_7 + \partial_r K_2 F_8 + \partial_{rr} B F_{10})) + A^3 \left( F_8 - B^3 (K_2 F_6 + \partial_r K_2 F_{10}) + B^2 \left( \partial_r v F_5 + K_1^2 F_7 - g_{JK_1} \kappa_g F_7 + 2 K_2^2 F_8 - g_{JK_2} \kappa_g F_8 + K_1 K_2 (2 F_7 + F_8) - \partial_r B K_2 F_{10} \right) \right) \right) \alpha +$$

$$\frac{1}{\tilde{A}^3 \tilde{B}^2} \left( -\tilde{A}^4 \tilde{B}^2 \tilde{K}_1 F_1 + \partial_r \tilde{A} \partial_r \tilde{B} \tilde{B} (2 F_3 + F_4) + \tilde{A} \left( -(\partial_r \tilde{B})^2 F_4 - \partial_{rr} \tilde{B} \tilde{B} (2 F_3 + F_4) + \partial_r \tilde{A} \partial_r \tilde{B} v \tilde{B}^2 F_9 \right) - \tilde{A}^2 \tilde{B}^2 (\partial_r v \partial_r \tilde{B} F_9 + v (\partial_r \tilde{B} F_2 + \partial_r \tilde{K}_1 F_3 + \partial_r \tilde{K}_2 F_4 + \partial_{rr} \tilde{B} F_9)) - \tilde{A}^3 \left( -F_4 + \tilde{B}^3 (\tilde{K}_2 F_2 + \partial_r \tilde{K}_2 F_9) + \tilde{B}^2 \left( \partial_r v F_1 + f_{JK_1} \kappa_f F_3 - \tilde{K}_1^2 F_3 + f_{JK_2} \kappa_f F_4 - 2 \tilde{K}_2^2 F_4 - \tilde{K}_1 \tilde{K}_2 (2 F_3 + F_4) + \partial_r \tilde{B} \tilde{K}_2 F_9 \right) \right) \right) \tilde{\alpha}$$

## Expand and recollect the terms factored by the lapses and their derivatives

```

corr$factor = fA fB^2 gA;
step$5 = step$4 * corr$factor /. Framed -> Identity /. F -> Fvalue // Expand;
factor$5 = factor$2 * corr$factor;

```

Factorize the expression over the derivatives of  $\alpha$  and  $\tilde{\alpha}$  (here we must include the contribution of the stress-energy tensor projections, both bimetric and matter; the matter contributions will be defined later),

```

Clear[nG, G, Gvalue];
nG = 0;
step$6 = step$5 /. {
  g$JK1 → eq$gV$JK1 + gT$JK1,
  g$JK2 → eq$gV$JK2 + gT$JK2,
  f$JK1 → eq$fV$JK1 + fT$JK1,
  f$JK2 → eq$fV$JK2 + fT$JK2,
  v → p / Lt
} // Expand // Collect[#, {
  gAlp[t_, r_], fAlp[t_, r_],
  Derivative[0, n_][gAlp][t_, r_],
  Derivative[0, n_][fAlp][t_, r_]
},
  (nG = nG + 1; Gvalue[nG] = Simplify@#; G[nG]) &
] &;

```

The following step requires **human intervention!**

```

step$6 // printNice // Framed
If[False, Do[Echo@Row@printNice@{G[n], " == ", Gvalue[n]}, {n, nG}]];
If[nG ≠ 5, FrontEndExecute[FrontEndToken["EvaluatorAbort"]]]

```

$$\alpha \mathbb{G}_1 + \tilde{\alpha} \mathbb{G}_2 + \partial_r \alpha \mathbb{G}_3 + \partial_r \tilde{\alpha} \mathbb{G}_4 + \mathbb{G}_5$$

The factors next to lapses should be appropriately named (done below). Note that there should be no second derivatives in lapses.

```

G$gAlp = Gvalue[1];
G$fAlp = Gvalue[2];
G$gAlp$r = Gvalue[3];
G$fAlp$r = Gvalue[4];
G$1 = Gvalue[5];

```

## Verify that there are no derivatives of the lapses

```

G$gAlp$r == 0 /. {Framed → Identity,
  Lt² → 1 + p², Lt$r$rule, R → fB / gB, esP$rule
} // Simplify;
% // printNice // Framed

```

True

```

G$fAlp$r == 0 /. {Framed → Identity,
  Lt² → 1 + p², Lt$r$rule, R → fB / gB, esP$rule
} // Simplify;
% // printNice // Framed

```

True

## The term which contains only $q$ and $\partial_r q$ also vanishes

At first, it looks quite complicated,

```

G$1 
$$\frac{1}{\mathbf{p}[2, 1, \mathbf{R}] \mathbf{qA} \mathbf{fA} \mathbf{qB}^3 \mathbf{R}^2} // . \{ \mathbf{Framed} \rightarrow \mathbf{Identity}, \mathbf{fB} \rightarrow \mathbf{qB} \mathbf{R} \} //$$

Collect[#, {q, D[q, r]}, Framed@Simplify@Expand@# &] &;
% // printNice

```

$$\mathbf{A} \mathbf{B} \lambda^2 \tilde{\mathbf{A}} \left( 2 \partial_r \tilde{\mathbf{B}} \langle \mathbf{R} \rangle_1^1 \mathbf{A}^2 \mathbf{p} \lambda + \lambda \tilde{\mathbf{A}}^2 \left( 2 \partial_r \mathbf{B} \langle \mathbf{R} \rangle_2^1 \mathbf{p} + \mathbf{A} \mathbf{B} \left( -2 \langle \mathbf{R} \rangle_2^1 \lambda \mathbf{K}_2 + \langle \mathbf{R} \rangle_1^2 \tilde{\mathbf{K}}_1 \right) + 2 \left( -\langle \mathbf{R} \rangle_1^1 + \langle \mathbf{R} \rangle_1^2 \right) \mathbf{A} \mathbf{B} \tilde{\mathbf{K}}_2 \right) + \right. \\ \left. \mathbf{A} \mathbf{B} \tilde{\mathbf{A}} \left( \partial_r \mathbf{p} \langle \mathbf{R} \rangle_1^2 + \mathbf{A} \lambda \left( -\langle \mathbf{R} \rangle_1^2 \mathbf{K}_1 - 2 \langle \mathbf{R} \rangle_1^1 \mathbf{K}_2 + 2 \langle \mathbf{R} \rangle_1^1 \mathbf{R} \lambda \tilde{\mathbf{K}}_2 \right) \right) \right)$$

$\partial_r \mathbf{q} +$

$$\begin{aligned} & -2 \partial_r \tilde{\mathbf{A}} \partial_r \tilde{\mathbf{B}} \langle \mathbf{R} \rangle_1^1 \mathbf{A}^3 \mathbf{p} \lambda^3 + \\ & 2 \mathbf{A}^2 \left( \partial_r \mathbf{A} \partial_r \tilde{\mathbf{B}} \langle \mathbf{R} \rangle_1^1 \mathbf{B} \mathbf{p} + \mathbf{A} \left( \partial_r \mathbf{p} \partial_r \tilde{\mathbf{B}} \langle \mathbf{R} \rangle_1^1 \mathbf{B} + \mathbf{p} \left( \langle \mathbf{R} \rangle_1^1 \left( -\partial_r \mathbf{B} \partial_r \tilde{\mathbf{B}} + \partial_{rr} \tilde{\mathbf{B}} \mathbf{B} \right) + \partial_r \tilde{\mathbf{B}} \langle \mathbf{R} \rangle_2^0 \left( \partial_r \tilde{\mathbf{B}} - \partial_r \mathbf{B} \mathbf{R} \right) \right) \right) \right) \lambda^3 \tilde{\mathbf{A}} + \\ & \lambda^2 \tilde{\mathbf{A}}^3 \left( -2 \partial_r \mathbf{A} \partial_r \mathbf{B} \langle \mathbf{R} \rangle_2^1 \mathbf{B} \mathbf{p} \lambda + 2 \mathbf{A} \left( \partial_r \mathbf{B} \partial_r \mathbf{p} \langle \mathbf{R} \rangle_2^1 \mathbf{B} + \mathbf{p} \left( \langle \mathbf{R} \rangle_2^1 \left( -(\partial_r \mathbf{B})^2 + \partial_{rr} \mathbf{B} \mathbf{B} \right) + \partial_r \mathbf{B} \langle \mathbf{R} \rangle_3^0 \left( \partial_r \tilde{\mathbf{B}} - \partial_r \mathbf{B} \mathbf{R} \right) \right) \right) \right) \\ & \lambda + \mathbf{A}^2 \mathbf{B} \left( -2 \left( \partial_r \mathbf{p} \langle \mathbf{R} \rangle_2^1 \mathbf{B} \mathbf{p} + \langle \mathbf{R} \rangle_2^0 \left( \partial_r \tilde{\mathbf{B}} - \partial_r \mathbf{B} \mathbf{R} \right) \lambda^2 \right) \mathbf{K}_2 + \right. \\ & \left. \lambda \left( \mathbf{B} \left( \left( \partial_r \tilde{\mathbf{K}}_1 + 2 \partial_r \tilde{\mathbf{K}}_2 \right) \langle \mathbf{R} \rangle_1^2 - 2 \left( \partial_r \tilde{\mathbf{K}}_2 \langle \mathbf{R} \rangle_1^1 + \partial_r \mathbf{K}_2 \langle \mathbf{R} \rangle_2^1 \lambda \right) \right) + 2 \langle \mathbf{R} \rangle_2^1 \left( \partial_r \tilde{\mathbf{B}} - \partial_r \mathbf{B} \mathbf{R} \right) \tilde{\mathbf{K}}_1 \right) \right) - \\ & 2 \left( \langle \mathbf{R} \rangle_2^0 - 2 \langle \mathbf{R} \rangle_2^1 \right) \mathbf{A}^2 \mathbf{B} \left( \partial_r \tilde{\mathbf{B}} - \partial_r \mathbf{B} \mathbf{R} \right) \lambda \tilde{\mathbf{K}}_2 + \mathbf{A} \mathbf{B} \tilde{\mathbf{A}}^2 \left( 2 \partial_r \mathbf{B} \partial_r \tilde{\mathbf{A}} \langle \mathbf{R} \rangle_2^1 \mathbf{p} \lambda^3 + \mathbf{A}^2 \lambda^3 \right. \\ & \left. \left( \mathbf{B} \left( -2 \partial_r \mathbf{K}_2 \langle \mathbf{R} \rangle_1^1 - \partial_r \mathbf{K}_1 \langle \mathbf{R} \rangle_1^2 + 2 \partial_r \tilde{\mathbf{K}}_2 \langle \mathbf{R} \rangle_1^1 \mathbf{R} \lambda \right) - 2 \langle \mathbf{R} \rangle_2^1 \left( \partial_r \tilde{\mathbf{B}} - \partial_r \mathbf{B} \mathbf{R} \right) \mathbf{K}_1 - 2 \langle \mathbf{R} \rangle_2^0 \left( \partial_r \tilde{\mathbf{B}} - \partial_r \mathbf{B} \mathbf{R} \right) \mathbf{K}_2 \right) - \right. \\ & \left. \mathbf{A} \left( -2 \partial_r \mathbf{p} \langle \mathbf{R} \rangle_2^1 \left( \partial_r \tilde{\mathbf{B}} - \partial_r \mathbf{B} \mathbf{R} \right) \lambda^2 + \right. \right. \\ & \left. \left. \mathbf{B} \left( 2 \lambda^3 \left( \partial_r \mathbf{A} \langle \mathbf{R} \rangle_1^1 + \partial_r \tilde{\mathbf{A}} \langle \mathbf{R} \rangle_2^1 \lambda \right) \mathbf{K}_2 + \langle \mathbf{R} \rangle_1^2 \left( (\partial_r \mathbf{p})^2 \mathbf{p} - \partial_{rr} \mathbf{p} \lambda^2 + \partial_r \mathbf{A} \lambda^3 \mathbf{K}_1 - \partial_r \tilde{\mathbf{A}} \lambda^3 \tilde{\mathbf{K}}_1 \right) \right) \right) + 2 \mathbf{A} \lambda^2 \right. \\ & \left. \left( \mathbf{A} \left( \partial_r \tilde{\mathbf{B}} - \partial_r \mathbf{B} \mathbf{R} \right) \left( \langle \mathbf{R} \rangle_1^1 + \langle \mathbf{R} \rangle_2^0 \mathbf{R} \right) \lambda^2 + \mathbf{B} \left( \partial_r \mathbf{p} \langle \mathbf{R} \rangle_1^1 \mathbf{A} \mathbf{p} \mathbf{R} + \partial_r \tilde{\mathbf{A}} \left( -\langle \mathbf{R} \rangle_1^1 + \langle \mathbf{R} \rangle_1^2 \right) \lambda + \partial_r \mathbf{A} \langle \mathbf{R} \rangle_1^1 \mathbf{R} \lambda^2 \right) \right) \tilde{\mathbf{K}}_2 \right) \end{aligned}$$

$\mathbf{q}$

It looks complicated even for  $\beta_1$ ,

```

G$1$forβ1 = G$1 
$$\frac{1}{\mathbf{qA}^3 \mathbf{qB}^3 \mathbf{fA}^3 \mathbf{fB}^2 \mathbf{Lt}^3} // . \{ \mathbf{Framed} \rightarrow \mathbf{Identity},$$


$$\mathbf{R} \rightarrow \mathbf{fB} / \mathbf{qB}, \mathbf{esP} \rightarrow \mathbf{rule}, \beta[2] \rightarrow 0, \beta[3] \rightarrow 0$$


$$\} // \text{Collect}[\#, \{\mathbf{q}, \mathbf{D}[\mathbf{q}, \mathbf{r}], \mathbf{p}, \mathbf{Lt}\}, \mathbf{Framed@Simplify@Expand@\# \&}] \&;$$

% // printNice

```

$$\begin{aligned} & \partial_r \mathbf{q} \left( \left( -\mathbf{A} (\mathbf{K}_1 + 2 \mathbf{K}_2) + \tilde{\mathbf{A}} \tilde{\mathbf{K}}_1 \right) \beta_1^2 \right) + \left( \frac{2 \partial_r \tilde{\mathbf{B}} \mathbf{A} \beta_1^2}{\mathbf{B} \tilde{\mathbf{A}}} \mathbf{p} + \frac{\partial_r \mathbf{p} \beta_1^2}{\lambda} + \frac{2 \mathbf{A} \tilde{\mathbf{B}} \tilde{\mathbf{K}}_2 \beta_1^2}{\mathbf{B}} \lambda \right) + \\ & \mathbf{q} \left( \frac{1}{\mathbf{B} \tilde{\mathbf{A}}} \left( 2 \partial_r \mathbf{p} \partial_r \tilde{\mathbf{B}} \mathbf{A} + \partial_r \tilde{\mathbf{K}}_1 \mathbf{B} \tilde{\mathbf{A}}^2 + \mathbf{B} \tilde{\mathbf{A}} \left( -\partial_r \mathbf{K}_1 \mathbf{A} - 2 \partial_r \mathbf{K}_2 \mathbf{A} - \partial_r \mathbf{A} \mathbf{K}_1 - 2 \partial_r \mathbf{A} \mathbf{K}_2 + \partial_r \tilde{\mathbf{A}} \tilde{\mathbf{K}}_1 \right) \right) \beta_1^2 + \right. \\ & \mathbf{p} \left( \frac{1}{\mathbf{B}^2 \tilde{\mathbf{A}}^2} 2 \left( \partial_r \mathbf{A} \partial_r \tilde{\mathbf{B}} \mathbf{B} \tilde{\mathbf{A}} - \mathbf{A} \left( \partial_r \mathbf{B} \partial_r \tilde{\mathbf{B}} \tilde{\mathbf{A}} + \mathbf{B} \left( \partial_r \tilde{\mathbf{A}} \partial_r \tilde{\mathbf{B}} - \partial_{rr} \tilde{\mathbf{B}} \tilde{\mathbf{A}} \right) \right) \right) \beta_1^2 + \frac{-(\partial_r \mathbf{p})^2 \beta_1^2}{\lambda^3} + \frac{2 \partial_r \mathbf{p} \mathbf{A} \tilde{\mathbf{B}} \tilde{\mathbf{K}}_2 \beta_1^2}{\lambda} \right) + \\ & \left. \frac{\partial_{rr} \mathbf{p} \beta_1^2}{\lambda} + \frac{2 \left( \partial_r \tilde{\mathbf{K}}_2 \mathbf{A} \mathbf{B} \tilde{\mathbf{B}} + \left( \partial_r \mathbf{A} \mathbf{B} \tilde{\mathbf{B}} + \mathbf{A} \left( \partial_r \tilde{\mathbf{B}} \mathbf{B} - \partial_r \mathbf{B} \tilde{\mathbf{B}} \right) \right) \tilde{\mathbf{K}}_2 \right) \beta_1^2}{\mathbf{B}^2} \lambda \right) \end{aligned}$$

However,  $\mathbf{G} \$ 1 \$ \mathbf{for} \beta 1$  is a total derivative of  $q$  multiplying the bimetric conservation law!



```

-β[1] q[t, r] eq$bimConsLaw[t, r] /. {R → fB / gB, esP$rule, β[2] → 0, β[3] → 0} // Expand;
% // printNice
D[%, r] == G$1$forβ1 /. {Framed → Identity, Lt$r$rule} // Simplify // printNice // Framed

$$\frac{\partial_r p q \beta_1^2}{\lambda} + \frac{2 \partial_r \tilde{B} A p q \beta_1^2}{B \tilde{A}} - A q K_1 \beta_1^2 - 2 A q K_2 \beta_1^2 + q \tilde{A} \tilde{K}_1 \beta_1^2 + \frac{2 A q \lambda \tilde{B} \tilde{K}_2 \beta_1^2}{B}$$

True

```

Below is the proof that this holds in general (and not only for  $\beta_1$ ).

```

q[t, r] eq$bimConsLaw[t, r] /. {R → fB / gB, esP$rule} // Expand;
D[%, r] // Expand;
factor$5-1 * G$1 /. {R → fB / gB, esP$rule} // Expand;
% == %% /. Lt$r$rule // Framed
True

```

Here we used the current overall factor in front of  $\mathbb{G}_1$ . This means that:

$$\partial_t C_{(\text{bim})} = \dots + \partial_r (q C_{(\text{bim})})$$

In fact, this should be obvious since we could gauge fix  $q = 0$  from the very beginning (in which case  $\mathbb{G}_1$  would vanish identically). Note that  $gW$  and  $fW$  do not depend on  $q$ .

**At this point, we have the factors in  $\alpha W_g + \tilde{\alpha} W_f = 0$ .**

## Eliminate the second derivatives

The second derivatives of  $B$  can be eliminated using the scalar constraints.

```
rule$secDerivativesOfB = Join[
  Solve[eq$gC$p == k$g (eq$gV$p + gT$p), Derivative[0, 2][gB][t, r][[1]],
  Solve[eq$fC$p == k$f (eq$fV$p + fT$p), Derivative[0, 2][fB][t, r][[1]]
] // Collect[#, {D[gB, r], D[fB, r], D[gK2, r], D[fK2, r]}, Simplify@Expand@# &] &;
Echo@printNice@# & /@%;

»  $\partial_{rr} B \rightarrow \frac{\partial_r A \partial_r B}{A} - \frac{(\partial_r B)^2}{2 B} + \frac{1}{2 B} A \left( \langle R \rangle_1^2 B^2 \lambda \tilde{A} \kappa_g + A \left( 1 + B^2 \left( 2 K_1 K_2 + K_2^2 + \langle R \rangle_0^2 \kappa_g - T \rho \kappa_g \right) \right) \right)$ 

»  $\partial_{rr} \tilde{B} \rightarrow \frac{\partial_r \tilde{A} \partial_r \tilde{B}}{\tilde{A}} - \frac{(\partial_r \tilde{B})^2}{2 \tilde{B}} + \frac{1}{2 R^2 \tilde{B}} \tilde{A} \left( R^2 \tilde{A} + \tilde{B}^2 \left( \langle R \rangle_1^2 A \lambda \kappa_f + \tilde{A} \left( \langle R \rangle_2^2 \kappa_f + R^2 \left( -\tilde{T} \rho \kappa_f + 2 \tilde{K}_1 \tilde{K}_2 + \tilde{K}_2^2 \right) \right) \right) \right)$ 
```

**Note:** We divide  $\mathbb{G}\$gAlp$  and  $\mathbb{G}\$fAlp$  by some factor and adjust the overall factor. We also get rid of all odd powers of  $Lt$  greater than one.

```
corr$factor =  $\frac{2}{gB^3 gA fA}$ ;

factor$final = factor$5 * corr$factor //.
  {fB → R gB, Lt^2 → 1 + p^2, Lt^3 → Lt (1 + p^2), Lt^4 → (1 + p^2)^2} // Simplify;
factor$final // printNice

 $2 \langle R \rangle_1^2 A^2 B^2 (1 + p^2) R^2 \lambda \tilde{A}^2$ 

temp = Block[{v}, v[t_, r_] := p[t, r] / Lt[t, r];
  G$gAlp * corr$factor //. {Framed → Identity,
    Sequence @@ rule$secDerivativesOfB, Lt$r$rule,
    D[R, r] → D[fB / gB, r]
  } // Expand
];

Collect[% //. {fB → R gB, Lt^2 → 1 + p^2, Lt^3 → Lt (1 + p^2), Lt^4 → (1 + p^2)^2}, {gB},
  Collect[#, {k$g, k$f}, Simplify] &];

eq$gW = Collect[% //. {fB → R gB, Lt^2 → 1 + p^2, Lt^3 → Lt (1 + p^2), Lt^4 → (1 + p^2)^2}, {gB},
  Collect[#, {k$g, k$f}, FullSimplify] &] /. {p + p^3 → p (1 + p^2), p^2 + p^4 → p^2 (1 + p^2)};

Block[{v}, v[t_, r_] := p[t, r] / Lt[t, r];
  G$fAlp * corr$factor /. {Framed → Identity,
    Sequence @@ rule$secDerivativesOfB, Lt$r$rule,
    D[R, r] → D[fB / gB, r]
  } // Expand
];

Collect[% //. {fB → R gB, Lt^2 → 1 + p^2, Lt^3 → Lt (1 + p^2), Lt^4 → (1 + p^2)^2}, {gB},
  Collect[#, {k$g, k$f}, Simplify] &];

eq$fW = Collect[% //. {fB → R gB, Lt^2 → 1 + p^2, Lt^3 → Lt (1 + p^2), Lt^4 → (1 + p^2)^2}, {gB},
  Collect[#, {k$g, k$f}, FullSimplify] &] /. {p + p^3 → p (1 + p^2), p^2 + p^4 → p^2 (1 + p^2)};
```

# Eliminate the first derivatives

The first derivatives of  $K_2$  can be eliminated using the j projection of  $V_g + V_f = V$ .

$$\underline{gA} \underline{gB}^2 \underline{eq\$gV\$j} + \underline{fA} \underline{fB}^2 \underline{eq\$fV\$j} == 0$$

True

```
rule$firstDerivativesOfK2 = Join[
  Solve[eqn$gC$j == k$g (eq$gV$j + gT$j), D[gK2, r]] [[1]],
  Solve[eqn$fC$j == k$f (eq$fV$j + fT$j), D[fK2, r]] [[1]]
] // Collect[#, {D[gB, r], D[fB, r]}, Simplify@Expand@# &] &;
Echo@printNice@# & /@%;
```

$$\gg \partial_r K_2 \rightarrow \frac{\partial_r B (K_1 - K_2)}{B} + \frac{1}{2} \left( -T_j \kappa_g + \langle R \rangle_1^2 p \tilde{A} \kappa_g \right)$$

$$\gg \partial_r \tilde{K}_2 \rightarrow \frac{1}{2} \left( -\frac{\langle R \rangle_1^2 A B^2 p}{\tilde{B}^2} - \tilde{T}_j \right) \kappa_f + \frac{\partial_r \tilde{B} (\tilde{K}_1 - \tilde{K}_2)}{\tilde{B}}$$

```
rule$derivativeOfp = Solve[0 == eq$bimConsLaw, D[p, r]] [[1]] //
  Collect[#, {D[gB, r], D[fB, r]}, Simplify@Expand@# &] &;
rule$derivativeOfp // printNice
```

$$\left\{ \partial_r p \rightarrow -\frac{2 \partial_r \tilde{B} \langle R \rangle_1^1 A p \lambda}{\langle R \rangle_1^2 B \tilde{A}} - \frac{2 \partial_r B \langle R \rangle_2^1 p \lambda \tilde{A}}{\langle R \rangle_1^2 A B} + \right. \\ \left. \frac{\lambda \left( \tilde{A} \left( 2 \langle R \rangle_2^1 \lambda K_2 - \langle R \rangle_1^2 \tilde{K}_1 + 2 \left( \langle R \rangle_1^1 - \langle R \rangle_1^2 \right) \tilde{K}_2 \right) + A \left( \langle R \rangle_1^2 K_1 + 2 \langle R \rangle_1^1 K_2 - 2 \langle R \rangle_1^1 R \lambda \tilde{K}_2 \right) \right)}{\langle R \rangle_1^2} \right\}$$

```

Block[{v}, v[t_, r_] := p[t, r] / Lt[t, r];
G$gAlp * corr$factor /. {Framed → Identity,
  Sequence @@ rule$secDerivativesOfB, Sequence @@ rule$firstDerivativesOfK2, Lt$r$rule,
  D[R, r] → D[fB / gB, r], Sequence @@ rule$derivativeOfp
} // Expand
];
Collect[% /. {fB → R gB} // Expand, {gB}, Simplify];
% /. {-1 - p^2 + Lt^2 → 0, -p^2 + Lt^2 → 1, -1 + p^2 + Lt^2 → 2 p^2,
  p^2 - Lt^2 → -1, 1 + p^2 → Lt^2, 4 p^2 - 4 Lt^2 → -4, -2 p^2 + 4 Lt^2 → 2 p^2 + 4};
eq$gW2 = Collect[%, {D[p, r], D[gB, r], D[fB, r]},
  Sequence @@ rule$firstDerivativesOfK2[[All, 1]]],
  Expand@Collect[#, {k$g, k$f}, Framed@Simplify@# &] &] // Expand;
eq$gW2 /. {k$g → Framed[k$g, Background → LightBlue],
  k$f → Framed[k$f, Background → LightRed]} // printNice
eq$gW2 = eq$gW2 /. Framed → Identity;

```

$$2 A^2 R \lambda^2 \tilde{A}^2 \left( \tilde{A} \left( 4 \left( \langle R \rangle_1^1 \right)^2 B^2 R^2 \tilde{K}_2^2 + R \left( 4 \left( \langle R \rangle_2^2 \right)^2 B^2 R \lambda^2 K_2^2 - \langle R \rangle_1^1 \langle R \rangle_2^1 \left( 1 + B^2 \left( -p^2 + 3 \lambda^2 \right) K_2^2 \right) - 2 \langle R \rangle_1^2 B^2 R \lambda K_2 \right. \right. \right. \\ \left. \left. \left( \langle R \rangle_3^0 \lambda K_2 + \langle R \rangle_2^0 \tilde{K}_2 \right) \right) + \langle R \rangle_1^1 \left( -4 \langle R \rangle_2^1 B^2 R K_2 \left( p^2 K_2 - 2 R \lambda \tilde{K}_2 \right) + \langle R \rangle_1^2 \left( 1 - 3 B^2 R^2 \tilde{K}_2^2 \right) \right) \right) + \\ A R \lambda \left( 4 \left( \langle R \rangle_1^1 \right)^2 B^2 R \tilde{K}_2 \left( \lambda K_2 - R \tilde{K}_2 \right) + \langle R \rangle_1^2 \left( \langle R \rangle_1^1 \left( 1 + B^2 K_2^2 \right) - 2 \langle R \rangle_2^0 B^2 R K_2 \left( K_2 - R \lambda \tilde{K}_2 \right) \right) - \right. \\ \left. 2 \langle R \rangle_1^1 \left( -2 \langle R \rangle_2^1 B^2 R K_2 \left( K_2 - R \lambda \tilde{K}_2 \right) + \langle R \rangle_1^2 \left( 1 + B^2 K_2 \left( 2 K_2 - R \lambda \tilde{K}_2 \right) \right) \right) \right) \right) +$$

$$\langle R \rangle_1^2 A^2 B^2 \lambda^2 \tilde{A}^2 \left( 6 \langle R \rangle_1^1 \langle R \rangle_1^2 A R \lambda + \tilde{A} \left( \langle R \rangle_1^2 \left( \langle R \rangle_1^2 + 2 \langle R \rangle_2^1 R \right) - 2 \langle R \rangle_1^1 \left( \langle R \rangle_1^2 - \langle R \rangle_2^2 R + R^3 \tilde{T} \rho \right) \right) \right) \mathcal{K}_f +$$

$$\langle R \rangle_1^2 A B^2 R^2 \lambda^2 \tilde{A}^2 \left( -4 \langle R \rangle_0^0 \langle R \rangle_1^1 A^2 \lambda - 4 \langle R \rangle_1^1 \langle R \rangle_1^2 A \tilde{A} + \left( \langle R \rangle_1^2 \right)^2 A \tilde{A} + 4 \langle R \rangle_2^1 p T_j \lambda \tilde{A} + \right. \\ \left. 2 \langle R \rangle_1^2 A^2 \lambda \left( -\langle R \rangle_0^0 + \langle R \rangle_0^2 - T \rho + T J_1 \right) + 4 \langle R \rangle_1^1 A^2 \lambda T J_2 - 2 \langle R \rangle_2^1 A \tilde{A} \left( \langle R \rangle_0^0 + T \rho \left( p^2 + \lambda^2 \right) - 2 \lambda^2 T J_2 \right) \right)$$

$$\mathcal{K}_g +$$

$$4 A B p R^2 \lambda^2 \tilde{A}^2 \left( A R \left( -2 \left( \langle R \rangle_1^1 \right)^2 - \langle R \rangle_1^2 \langle R \rangle_2^0 R - \langle R \rangle_1^1 \left( \langle R \rangle_1^2 - 2 \langle R \rangle_2^1 R \right) \right) \lambda \tilde{K}_2 + \right. \\ \left. \tilde{A} \left( 2 \left( 2 \langle R \rangle_1^1 \langle R \rangle_2^1 + \langle R \rangle_1^2 \langle R \rangle_2^1 - 2 \left( \langle R \rangle_2^2 \right)^2 R + \langle R \rangle_1^2 \langle R \rangle_3^0 R \right) \lambda K_2 + \left( \langle R \rangle_1^2 \langle R \rangle_2^0 - 4 \langle R \rangle_1^1 \langle R \rangle_2^1 \right) R \tilde{K}_2 \right) \right) \partial_r B +$$

$$2 R^2 \lambda^2 \tilde{A}^2 \left( A \left( -\langle R \rangle_1^2 \left( \langle R \rangle_1^2 - 2 \langle R \rangle_2^0 R \right) + 4 \langle R \rangle_1^1 \left( \langle R \rangle_1^2 - \langle R \rangle_2^1 R \right) \right) \lambda + \right. \\ \left. \left( p^2 \left( -3 \langle R \rangle_1^2 \langle R \rangle_2^1 + 4 \left( \langle R \rangle_2^2 \right)^2 R - 2 \langle R \rangle_1^2 \langle R \rangle_3^0 R \right) + \left( -4 \langle R \rangle_1^1 + \langle R \rangle_1^2 \right) \langle R \rangle_2^1 \lambda^2 \right) \tilde{A} \right) (\partial_r B)^2 +$$

$$4 A^2 B p R^2 \lambda \tilde{A} \\ \left( A \left( 2 \left( \langle R \rangle_1^1 \right)^2 \left( 1 + p^2 \right) + \langle R \rangle_1^2 \langle R \rangle_2^0 R \lambda^2 + \langle R \rangle_1^1 \left( \langle R \rangle_1^2 - 2 \langle R \rangle_2^1 R \right) \lambda^2 \right) + \left( \langle R \rangle_1^2 \langle R \rangle_2^0 - 4 \langle R \rangle_1^1 \langle R \rangle_2^1 \right) \lambda \tilde{A} \right) K_2$$

$$\partial_r \tilde{B} + \left( -4 A R^2 \lambda^3 \tilde{A} \left( A \left( 2 \left( \langle R \rangle_1^1 \right)^2 + \langle R \rangle_1^2 \langle R \rangle_2^0 R + \langle R \rangle_1^1 \left( \langle R \rangle_1^2 - 2 \langle R \rangle_2^1 R \right) \right) \lambda + \left( \langle R \rangle_1^2 \langle R \rangle_2^0 - 4 \langle R \rangle_1^1 \langle R \rangle_2^1 \right) \tilde{A} \right) \right)$$

$$\partial_r B \partial_r \tilde{B} + \left( 2 A^2 R \lambda^2 \left( 4 \left( \langle R \rangle_1^1 \right)^2 A R \lambda - \left( -2 \langle R \rangle_1^2 \langle R \rangle_2^0 R + \langle R \rangle_1^1 \left( \langle R \rangle_1^2 + 4 \langle R \rangle_2^1 R \right) \right) \tilde{A} \right) \right) (\partial_r \tilde{B})^2$$

```

Block[{v}, v[t_, r_] := p[t, r] / Lt[t, r];
G$fAlp * corr$factor /. {Framed -> Identity,
  Sequence @@ rule$secDerivativesOfB, Sequence @@ rule$firstDerivativesOfK2, Lt$r$rule,
  D[R, r] -> D[fB / gB, r], Sequence @@ rule$derivativeOfp
} // Expand
];
Collect[%, /. {fB -> R gB} // Expand, {fB}, Simplify];
% /. {-1 - p^2 + Lt^2 -> 0, -p^2 + Lt^2 -> 1, -1 + p^2 + Lt^2 -> 2 p^2,
  p^2 - Lt^2 -> -1, 1 + p^2 - Lt^2 -> 4 p^2 - 4 Lt^2 -> -4, -2 p^2 + 4 Lt^2 -> 2 p^2 + 4};
eq$fW2 = Collect[%, {D[p, r], D[gB, r], D[fB, r]},
  Sequence @@ rule$firstDerivativesOfK2[All, 1]],
  Expand@Collect[#, {k$g, k$f}, Framed@Simplify@# &] // Expand;
eq$fW2 /. {k$g -> Framed[k$g, Background -> LightBlue],
  k$f -> Framed[k$f, Background -> LightRed]} // printNice
eq$fW2 = eq$fW2 /. Framed -> Identity;

```

$$\begin{aligned}
& 2 A^2 \lambda^2 \tilde{A}^2 \\
& \left( \lambda \tilde{A} \left( R \left( 2 \langle R \rangle_1^2 B^2 R \tilde{K}_2 \left( \langle R \rangle_3^0 R \lambda K_2 - \langle R \rangle_1^2 \tilde{K}_1 + \left( \langle R \rangle_1^2 + \langle R \rangle_2^0 R \right) \tilde{K}_2 \right) + 4 \left( \langle R \rangle_2^1 \right)^2 B^2 R K_2 \left( K_2 - R \lambda \tilde{K}_2 \right) + \right. \right. \right. \\
& \quad \left. \left. \left. \langle R \rangle_1^2 \langle R \rangle_2^1 \left( 1 + 2 B^2 R \left( -2 \lambda K_2 + R \tilde{K}_1 \right) \tilde{K}_2 + B^2 R^2 \tilde{K}_2^2 \right) \right) \right) - \right. \\
& \quad \left. \langle R \rangle_1^1 \left( 4 \langle R \rangle_2^1 B^2 R^2 \tilde{K}_2 \left( -\lambda K_2 + R \tilde{K}_2 \right) + \langle R \rangle_1^2 \left( 1 - 2 B^2 R^2 \tilde{K}_1 \tilde{K}_2 + 3 B^2 R^2 \tilde{K}_2^2 \right) \right) \right) + \\
& A R \left( \langle R \rangle_2^2 R \left( -\langle R \rangle_1^2 + \left( 4 \langle R \rangle_1^1 - \langle R \rangle_1^2 \right) B^2 K_2^2 \right) + 2 \left( \langle R \rangle_1^2 \langle R \rangle_2^0 - 4 \langle R \rangle_1^1 \langle R \rangle_2^1 \right) B^2 R^2 \lambda K_2 \tilde{K}_2 - \right. \\
& \quad \left. \langle R \rangle_1^1 p^2 \left( 4 \langle R \rangle_1^1 B^2 R^2 \tilde{K}_2^2 + \langle R \rangle_1^2 \left( 1 - 3 B^2 R^2 \tilde{K}_2^2 \right) \right) + \right. \\
& \quad \left. \lambda^2 \left( -2 \langle R \rangle_1^2 \langle R \rangle_2^0 B^2 R^3 \tilde{K}_2^2 + \langle R \rangle_1^1 \left( 4 \langle R \rangle_2^1 B^2 R^3 \tilde{K}_2^2 + \langle R \rangle_1^2 \left( 1 + B^2 R^2 \tilde{K}_2^2 \right) \right) \right) \right) \right) \Bigg) +
\end{aligned}$$

$$\begin{aligned}
& \langle R \rangle_1^2 A^2 B^2 \lambda^2 \tilde{A} \left( 4 \langle R \rangle_1^1 A p R^3 \lambda \tilde{T}j + A \tilde{A} \left( \langle R \rangle_1^2 \left( \langle R \rangle_1^2 \left( 1 - 2 \lambda^2 \right) + 2 \langle R \rangle_2^1 R \left( 1 + \lambda^2 \right) \right) + \right. \right. \\
& \quad \left. \left. 2 \langle R \rangle_1^1 \left( \langle R \rangle_1^2 \left( -1 + \lambda^2 \right) + R \left( p^2 \left( -\langle R \rangle_2^2 + R^2 \tilde{T}\rho \right) + \lambda^2 \left( \langle R \rangle_2^2 + R^2 \left( \tilde{T}\rho - 2 \tilde{T}j_2 \right) \right) \right) \right) \right) - 2 \lambda \tilde{A}^2 \right. \\
& \quad \left. \left( \langle R \rangle_1^1 \left( \langle R \rangle_2^2 + R^2 \left( \tilde{T}\rho - 2 \tilde{T}j_2 \right) \right) + R \left( -\langle R \rangle_1^2 \langle R \rangle_3^1 + \langle R \rangle_2^1 \left( -\langle R \rangle_2^2 + R^2 \tilde{T}\rho \right) + \langle R \rangle_1^2 R \left( -2 \tilde{T}\rho + \tilde{T}j_1 + 2 \tilde{T}j_2 \right) \right) \right) \right) \Bigg)
\end{aligned}$$

$$\kappa_f + \langle R \rangle_1^2 A^2 B^2 R^2 \lambda^2 \tilde{A}^2 \left( A \left( -4 \langle R \rangle_1^1 \langle R \rangle_1^2 + \left( \langle R \rangle_1^2 \right)^2 - 2 \langle R \rangle_2^0 \langle R \rangle_2^1 + 2 \langle R \rangle_2^1 T\rho \right) - 6 \langle R \rangle_1^2 \langle R \rangle_2^1 \lambda \tilde{A} \right)$$

$$\kappa_g + \left( 4 A B p R^2 \lambda \tilde{A}^2 \left( \left( \langle R \rangle_1^2 \langle R \rangle_2^0 - 4 \langle R \rangle_1^1 \langle R \rangle_2^1 \right) A R \lambda - \right. \right. \\
\left. \left. \left( 2 \langle R \rangle_1^2 \langle R \rangle_2^1 \left( 1 + p^2 \right) + \left( 2 \langle R \rangle_1^1 \langle R \rangle_2^1 - 4 \langle R \rangle_1^2 \langle R \rangle_2^1 - 2 \left( \langle R \rangle_2^1 \right)^2 R + \langle R \rangle_1^2 \langle R \rangle_3^0 R \right) \lambda^2 \right) \tilde{A} \right) \tilde{K}_2 \right) \partial_r B +$$

$$-2 R^2 \lambda^2 \tilde{A}^2 \left( A \left( -3 \langle R \rangle_1^2 \langle R \rangle_2^1 + 4 \left( \langle R \rangle_2^1 \right)^2 R - 2 \langle R \rangle_1^2 \langle R \rangle_3^0 R \right) + 4 \left( \langle R \rangle_2^1 \right)^2 \lambda \tilde{A} \right) \left( \partial_r B \right)^2 +$$

$$\left( 4 A^2 B p R^2 \lambda^2 \tilde{A} \left( \left( \left( \langle R \rangle_1^2 \langle R \rangle_2^0 - 4 \langle R \rangle_1^1 \langle R \rangle_2^1 \right) A + \left( -4 \left( \langle R \rangle_2^1 \right)^2 + \langle R \rangle_1^2 \langle R \rangle_3^0 \right) \lambda \tilde{A} \right) K_2 - \right. \right. \\
\left. \left. 2 A \left( \left( \langle R \rangle_1^1 \right)^2 + \langle R \rangle_1^2 \langle R \rangle_2^0 R - \langle R \rangle_1^1 \left( \langle R \rangle_1^2 + 3 \langle R \rangle_2^1 R \right) \right) \lambda \tilde{K}_2 \right) \right) \partial_r \tilde{B} +$$

$$-4 A R^2 \lambda^3 \tilde{A} \left( A \left( 2 \langle R \rangle_1^1 \langle R \rangle_2^1 + \langle R \rangle_1^2 \langle R \rangle_2^1 - 2 \left( \langle R \rangle_2^1 \right)^2 R + \langle R \rangle_1^2 \langle R \rangle_3^0 R \right) + \left( -4 \left( \langle R \rangle_2^1 \right)^2 + \langle R \rangle_1^2 \langle R \rangle_3^0 \right) \lambda \tilde{A} \right) \partial_r B$$

$$\partial_r \tilde{B} + \left( 2 A^2 \lambda^2 \left( A R \left( p^2 \left( -2 \langle R \rangle_1^2 \langle R \rangle_2^0 R + \langle R \rangle_1^1 \left( \langle R \rangle_1^2 + 4 \langle R \rangle_2^1 R \right) \right) - \langle R \rangle_1^1 \left( \langle R \rangle_1^2 - 4 \langle R \rangle_2^1 R \right) \lambda^2 \right) + \right. \right. \\
\left. \left. \left( \langle R \rangle_1^1 \langle R \rangle_2^1 - R \left( \langle R \rangle_1^2 \langle R \rangle_2^1 + 4 \left( \langle R \rangle_2^1 \right)^2 R - 2 \langle R \rangle_1^2 \langle R \rangle_3^0 R \right) \right) \lambda \tilde{A} \right) \right) \left( \partial_r \tilde{B} \right)^2$$

## Symmetry of $W_g$ and $W_f$

The two sectors are symmetric under the exchange  $g \leftrightarrow f$  of all the fields, in addition to  $p \leftrightarrow -p$  and  $\beta_n \leftrightarrow \beta_{4-n}$ . In such case  $W_{g \rightarrow f} = -W_f$ .

```

swapSectors[e_] :=
  R^-6 e /. {P[n_, k_, ev_] := eq$esP[n, k, ev]} /. {β[n_] := β[4 - n]} /. R → fB / gB /. {
    p → -p,
    gA → xA, gB → xB, gK1 → xK1, gK2 → xK2, gK → xK,
    fA → yA, fB → yB, fK1 → yK1, fK2 → yK2, fK → yK,
    gT$ρ → xT$ρ, gT$j → xT$j, gT$JK1 → xT$JK1, gT$JK2 → xT$JK2,
    fT$ρ → yT$ρ, fT$j → yT$j, fT$JK1 → yT$JK1, fT$JK2 → yT$JK2,
    k$g → k$x, k$f → k$y
  } /. {
    yA → gA, yB → gB, yK1 → gK1, yK2 → gK2, yK → gK,
    xA → fA, xB → fB, xK1 → fK1, xK2 → fK2, xK → fK,
    yT$ρ → gT$ρ, yT$j → gT$j, yT$JK1 → gT$JK1, yT$JK2 → gT$JK2,
    xT$ρ → fT$ρ, xT$j → fT$j, xT$JK1 → fT$JK1, xT$JK2 → fT$JK2,
    k$y → k$g, k$x → k$f
  } // Expand

swapped$gW = eq$gW2 // swapSectors;
actual$fW = eq$fW2 /. {P[n_, k_, ev_] := eq$esP[n, k, ev]} /. R → fB / gB // Expand;
swapped$gW == -actual$fW /. Lt → (1 + p^2)^1/2 // Expand // printNice

```

True

## Save the module “bimetric-lapses-nr.m”

```

defs = "";

appendDefs[name_, expr_] := (defs = defs <> name <> "[t_, r_] := " <>
  ToString@InputForm[expr] <> "\n\n");

appendDefs["eqn$gW", eq$gW]
appendDefs["eqn$fW", eq$fW]
appendDefs["eqn$gW2", eq$gW2]
appendDefs["eqn$fW2", eq$fW2]
appendDefs["eqn$cW", factor$final]

appendDefs["eqr$gW",
  Collect[eq$gW /. {gB[t_, r_] => gB[t, r] r, fB[t_, r_] => fB[t, r] r}, {r, k$g, k$f}, Simplify]]
appendDefs["eqr$fW",
  Collect[eq$fW /. {gB[t_, r_] => gB[t, r] r, fB[t_, r_] => fB[t, r] r}, {r, k$g, k$f}, Simplify]]
appendDefs["eqr$gW2", Collect[
  eq$gW2 /. {gB[t_, r_] => gB[t, r] r, fB[t_, r_] => fB[t, r] r}, {r, k$g, k$f}, Simplify]]
appendDefs["eqr$fW2", Collect[eq$fW2 /. {gB[t_, r_] => gB[t, r] r, fB[t_, r_] => fB[t, r] r},
  {r, k$g, k$f}, Simplify]]
appendDefs["eqr$cW", Collect[factor$final /.
  {gB[t_, r_] => gB[t, r] r, fB[t_, r_] => fB[t, r] r}, {r, k$g, k$f}, Simplify]]

Export["bimetric-lapses-nr.m", defs, "String"];

```
